# Supplementary material for: Pseudo-Goldstone gaps and order-by-quantum-disorder in frustrated magnets
Source: arXiv:1805.00947 source file (2018-11-12)
Supplement: Supplementary file 1 [file supp.pdf]

# Supplemental material for “Order-by-quantum-disorder and the fate of pseudo-Goldstone modes”

Jeffrey G. Rau, Paul A. McClarty, and Roderich Moessner

*Max-Planck-Institut für Physik komplexer Systeme, 01187 Dresden, Germany*

(Dated: November 12, 2018)

## CONTENTS

S1. Linear spin-wave theory 2
A. Zero modes 3

S2. Non-linear spin-wave theory 4
A. Pseudo-Goldstone modes 6

S3. Proof of curvature formula 7
A. Self-correcting linear spin-waves 7
B. First moment sum rule and spectral functions 10
C. Warm up: No pseudo-Goldstone mode 12
D. Type II pseudo-Goldstone mode 13
E. Type I pseudo-Goldstone mode 14

S4. Remarks on some connections to quantum chromodynamics 15

S5. Order-by-quantum disorder models 17
A. Heisenberg-compass models 17
B. Heisenberg-Kitaev-Γ models 17
C. $J_1$-$J_2$ models 18
D. $Ca_3Fe_2Ge_3O_{12}$ 19
E. $Er_2Ti_2O_7$ 20

S6. Curvature calculation examples 21
A. Heisenberg-compass (cubic, ferromagnet) 21
B. $J$-Γ model (honeycomb, ferromagnet) 22
C. Heisenberg $J_1$-$J_2$ (square, stripe) 22

S7. Worked example: Heisenberg-compass model on square lattice 23

References 26

## S1. LINEAR SPIN-WAVE THEORY

Consider a general translational invariant spin model

$$H \equiv \frac{1}{2}\sum_{\boldsymbol{r}\boldsymbol{r}'}\sum_{\alpha\alpha'} \boldsymbol{S}_{\boldsymbol{r}\alpha}{}^{\intercal}\boldsymbol{J}_{\boldsymbol{r}-\boldsymbol{r}',\alpha\alpha'}\boldsymbol{S}_{\boldsymbol{r}'\alpha'}, \tag{S1}$$

where $\boldsymbol{S}_{\boldsymbol{r}\alpha}$ is a spin-$S$ operator located in unit cell $\boldsymbol{r}$ with sublattice index $\alpha$. The spin operators can expressed in terms of Holstein-Primakoff bosons as

$$\boldsymbol{S}_{\boldsymbol{r}\alpha} \equiv \sqrt{S}\left[\left(1-\frac{n_{\boldsymbol{r}\alpha}}{2S}\right)^{1/2} a_{\boldsymbol{r}\alpha}\hat{\boldsymbol{e}}_{\alpha,-} + a^{\dagger}_{\boldsymbol{r}\alpha}\left(1-\frac{n_{\boldsymbol{r}\alpha}}{2S}\right)^{1/2}\hat{\boldsymbol{e}}_{\alpha,+}\right] + (S-n_{\boldsymbol{r}\alpha})\,\hat{\boldsymbol{e}}_{\alpha,0}, \tag{S2}$$

where $n_{\boldsymbol{r}\alpha} \equiv a^{\dagger}_{\boldsymbol{r}\alpha}a_{\boldsymbol{r}\alpha}$. The vectors $\hat{\boldsymbol{e}}_{\alpha,\pm}$, $\hat{\boldsymbol{e}}_{\alpha,0}$ define a local frame of reference; in a more conventional Cartesian basis one defines $\hat{\boldsymbol{e}}_{\alpha,\pm} \equiv (\hat{\boldsymbol{x}}_{\alpha} \pm i\hat{\boldsymbol{y}}_{\alpha})/\sqrt{2}$ and $\hat{\boldsymbol{e}}_{\alpha,0} \equiv \hat{\boldsymbol{z}}_{\alpha}$. It is useful to write the exchange matrix in this frame

$$\mathcal{J}^{\mu\mu'}_{\boldsymbol{\delta},\alpha\alpha'} \equiv \hat{\boldsymbol{e}}^{\intercal}_{\alpha,\mu}\boldsymbol{J}_{\boldsymbol{\delta},\alpha\alpha'}\hat{\boldsymbol{e}}_{\alpha',\mu'}. \tag{S3}$$

Expanding in powers of $1/S$ then yields a semi-classical expansion about the ordered state defined by $\hat{\boldsymbol{e}}_{\alpha,0}$, typically chosen to be along the classical ordering direction. In this case at order $O(S)$ in the Holstein-Primakoff operators one finds a quadratic form

$$H = NS(S+1)\epsilon_{\rm cl} + \frac{1}{2}S\sum_{\boldsymbol{k}}\left([\boldsymbol{a}^{\dagger}_{\boldsymbol{k}}]^{\intercal}\ \boldsymbol{a}^{\intercal}_{-\boldsymbol{k}}\right)\begin{pmatrix}\boldsymbol{A}_{\boldsymbol{k}} & \boldsymbol{B}_{\boldsymbol{k}}\\ \boldsymbol{B}^{\dagger}_{\boldsymbol{k}} & \boldsymbol{A}^{\intercal}_{-\boldsymbol{k}}\end{pmatrix}\begin{pmatrix}\boldsymbol{a}_{\boldsymbol{k}}\\ \boldsymbol{a}^{\dagger}_{-\boldsymbol{k}}\end{pmatrix} + O(S^{1/2}), \tag{S4}$$

where $N_s$ is the number of sublattices, $N$ is the total number of sites and we have defined the Fourier transforms of the bosons as $a_{\boldsymbol{k}\alpha} \equiv N_c^{-1/2}\sum_{\boldsymbol{r}} e^{-i\boldsymbol{k}\cdot\boldsymbol{r}}a_{\boldsymbol{r}\alpha}$ where $N = N_cN_s$. The classical energy per site is defined as

$$\epsilon_{\rm cl} \equiv \frac{1}{2N_s}\sum_{\alpha\alpha'}\sum_{\boldsymbol{\delta}}\mathcal{J}^{00}_{\boldsymbol{\delta},\alpha\alpha'}, \tag{S5}$$

and the matrices $\boldsymbol{A}_{\boldsymbol{k}}$ and $\boldsymbol{B}_{\boldsymbol{k}}$ are given by

$$A^{\alpha\alpha'}_{\boldsymbol{k}} = \mathcal{J}^{+-}_{\boldsymbol{k},\alpha\alpha'} - \delta_{\alpha\alpha'}\sum_{\mu}\mathcal{J}^{00}_{\boldsymbol{0},\alpha\mu}, \tag{S6a}$$

$$B^{\alpha\alpha'}_{\boldsymbol{k}} = \mathcal{J}^{++}_{\boldsymbol{k},\alpha\alpha'}, \tag{S6b}$$

where we have defined the Fourier transforms of the local exchange matrices as

$$\mathcal{J}^{\mu\mu'}_{\boldsymbol{k},\alpha\alpha'} \equiv \sum_{\boldsymbol{\delta}}\mathcal{J}^{\mu\mu'}_{\boldsymbol{\delta},\alpha\alpha'}e^{i\boldsymbol{k}\cdot\boldsymbol{\delta}}. \tag{S7}$$

The linear spin-wave Hamiltonian [Eq. (S4)] can be diagonalized by a Bogoliubov transformation. To do this one diagonalizes the modified matrix [1]

$$\begin{pmatrix}\boldsymbol{A}_{\boldsymbol{k}} & \boldsymbol{B}_{\boldsymbol{k}}\\ -\boldsymbol{B}^{\dagger}_{\boldsymbol{k}} & -\boldsymbol{A}^{\intercal}_{-\boldsymbol{k}}\end{pmatrix} \equiv \boldsymbol{\sigma}_3\boldsymbol{M}_{\boldsymbol{k}} \tag{S8}$$

This yields pairs of eigenvectors $\boldsymbol{V}_{\boldsymbol{k}\alpha}$ and $\boldsymbol{W}_{-\boldsymbol{k},\alpha} = \boldsymbol{\sigma}_1 \boldsymbol{V}^*_{-\boldsymbol{k}\alpha}$ with eigenvalues $+\epsilon_{\boldsymbol{k}\alpha}$ and $-\epsilon_{-\boldsymbol{k},\alpha}$. These vectors can be normalized such that [1]

$$\boldsymbol{V}^\dagger_{\boldsymbol{k}\alpha}\boldsymbol{\sigma}_3\boldsymbol{V}_{\boldsymbol{k}\alpha'} = +\delta_{\alpha\alpha'}, \qquad \boldsymbol{W}^\dagger_{-\boldsymbol{k}\alpha}\boldsymbol{\sigma}_3\boldsymbol{W}_{-\boldsymbol{k}\alpha'} = -\delta_{\alpha\alpha'}, \qquad \boldsymbol{W}^\dagger_{-\boldsymbol{k}\alpha}\boldsymbol{\sigma}_3\boldsymbol{V}_{\boldsymbol{k}\alpha'} = 0. \tag{S9}$$

One can then write the Hamiltonian in terms of diagonalized bosons, $\gamma_{\boldsymbol{k}\alpha}$, as [1]

$$H \equiv NS(S+1)\epsilon_{\rm cl} + NS\epsilon_{\rm qu} + S\sum_{\boldsymbol{k}\alpha}\epsilon_{\boldsymbol{k}\alpha}\gamma^\dagger_{\boldsymbol{k}\alpha}\gamma_{\boldsymbol{k}\alpha} + O(S^{1/2}), \tag{S10}$$

where we have identified the energy per site from quantum zero-point motion, $\epsilon_{\rm qu}$, as

$$\epsilon_{\rm qu} \equiv \frac{1}{2N}\sum_{\boldsymbol{k}\alpha}\epsilon_{\boldsymbol{k}\alpha} \tag{S11}$$

The diagonalized bosons can be related to the original Holstein-Primakoff bosons via the relations

$$\begin{pmatrix} \boldsymbol{\gamma}_{\boldsymbol{k}} \\ \boldsymbol{\gamma}^\dagger_{-\boldsymbol{k}} \end{pmatrix} = \begin{pmatrix} \boldsymbol{X}^*_{\boldsymbol{k}} & -\boldsymbol{Y}^*_{\boldsymbol{k}} \\ -\boldsymbol{Y}_{-\boldsymbol{k}} & \boldsymbol{X}_{-\boldsymbol{k}} \end{pmatrix}\begin{pmatrix} \boldsymbol{a}_{\boldsymbol{k}} \\ \boldsymbol{a}^\dagger_{-\boldsymbol{k}} \end{pmatrix} \equiv \boldsymbol{T}_{\boldsymbol{k}}\begin{pmatrix} \boldsymbol{a}_{\boldsymbol{k}} \\ \boldsymbol{a}^\dagger_{-\boldsymbol{k}} \end{pmatrix}. \tag{S12}$$

The matrices $\boldsymbol{X}_{\boldsymbol{k}}$ and $\boldsymbol{Y}_{\boldsymbol{k}}$ are defined in terms the $\boldsymbol{V}_{\boldsymbol{k}\alpha}$ and $\boldsymbol{W}_{-\boldsymbol{k},\alpha}$ vectors, with the columns of $\boldsymbol{T}^{-1}_{\boldsymbol{k}}$ being the $\boldsymbol{V}_{\boldsymbol{k}\alpha}$ followed by the $\boldsymbol{W}_{-\boldsymbol{k},\alpha}$ vectors.

### A. Zero modes

The diagonalization of $\boldsymbol{\sigma}_3\boldsymbol{M}_{\boldsymbol{k}}$ can be carried out straightforwardly if $\boldsymbol{M}_{\boldsymbol{k}}$ is positive definite. Since we are interested in linear spin-wave problem with zero modes, we must treat the case where it is only positive-*semi*-definite in detail, following Blaizot and Ripka [1].

Consider then the case where one has a single zero mode at $\boldsymbol{k} = \boldsymbol{0}$; there is no loss of generality so long as all zero modes occur at commensurate wave-vectors. Now, the matrix $\boldsymbol{M}_0$ is Hermitian, with $\boldsymbol{M}_0 = \boldsymbol{M}^\dagger_0$, and satisfies $\boldsymbol{\sigma}_1\boldsymbol{M}_0\boldsymbol{\sigma}_1 = \boldsymbol{M}^\intercal_0$. Since $\boldsymbol{M}_0$ and $\boldsymbol{\sigma}_0\boldsymbol{M}_0$ share zero modes, we classify the type of zero mode by the spectral properties of $\boldsymbol{M}_0$. There are two possibilities: $\boldsymbol{M}_0$ has a single zero eigenvector (type I) or $\boldsymbol{M}_0$ has two linearly independent zero eigenvectors (type II). We define vectors [1] that span the zero mode subspace as $\boldsymbol{V}_0$ and $\boldsymbol{W}_0$ for both type I and type II cases. These can be chosen [1] to satisfy the normalization conditions [Eq. (S9)]

$$\boldsymbol{V}^\dagger_0\boldsymbol{\sigma}_3\boldsymbol{V}_0 = +1, \qquad \boldsymbol{W}^\dagger_0\boldsymbol{\sigma}_3\boldsymbol{W}_0 = -1, \qquad \boldsymbol{V}^\dagger_0\boldsymbol{\sigma}_3\boldsymbol{W}_0 = 0, \tag{S13}$$

where $\boldsymbol{W}_0 = \boldsymbol{\sigma}_1\boldsymbol{V}^*_0$. It useful to define the block forms of these matrices

$$\boldsymbol{V}_0 \equiv \begin{pmatrix} \boldsymbol{X}_0 \\ \boldsymbol{Y}_0 \end{pmatrix}, \qquad \boldsymbol{W}_0 \equiv \begin{pmatrix} \boldsymbol{Y}^*_0 \\ \boldsymbol{X}^*_0 \end{pmatrix}. \tag{S14}$$

Their relationship with the dispersion matrix depends on the type of the zero mode. One has

$$\boldsymbol{M}_0\boldsymbol{V}_0 = \boldsymbol{M}_0\boldsymbol{W}_0 = \begin{cases} (2\mu)^{-1}\boldsymbol{\sigma}_3\left(\boldsymbol{V}_0 - \boldsymbol{W}_0\right), & \text{type I} \\ 0 & \text{type II} \end{cases}, \tag{S15}$$

where we have defined

$$\frac{1}{2\mu} \equiv \boldsymbol{V}_0^\dagger \boldsymbol{M}_0 \boldsymbol{V}_0. \tag{S16}$$

The case of a type I zero mode corresponds to $\boldsymbol{\sigma}_3 \boldsymbol{M}_0$ being non-diagonalizable, with the zero mode subspace being a two by two Jordan block. This can be seen by projecting the dispersion into the subspace spanned by $\boldsymbol{V}_0$ and $\boldsymbol{W}_0$, where one finds

$$\begin{pmatrix} \boldsymbol{V}_0^\dagger \boldsymbol{M}_0 \boldsymbol{V}_0 & \boldsymbol{V}_0^\dagger \boldsymbol{M}_0 \boldsymbol{W}_0 \\ \boldsymbol{W}_0^\dagger \boldsymbol{M}_0 \boldsymbol{V}_0 & \boldsymbol{W}_0^\dagger \boldsymbol{M}_0 \boldsymbol{W}_0 \end{pmatrix} = \frac{1}{2\mu} \begin{pmatrix} +1 & +1 \\ +1 & +1 \end{pmatrix} \text{ (type I)}, \quad \begin{pmatrix} 0 & 0 \\ 0 & 0 \end{pmatrix} \text{ (type II)}. \tag{S17}$$

Classically, a type I zero mode can be understood as a mode that costs zero energy, but its canonically conjugate partner costs finite energy; the type II case corresponds to both having zero energy cost.

## S2. NON-LINEAR SPIN-WAVE THEORY

Going to next order in $1/S$, one obtains a considerably more complex Hamiltonian. This can be written as a sum of the usual two-magnon terms, as well as three- and four-magnon interactions. We write

$$H = NS(S+1)\epsilon_{\rm cl} + S H_2 + S^{1/2} H_3 + S^0 H_4 \tag{S18}$$

where we define the individual pieces in symmetrized form as

$$H_2 = \frac{1}{2} \sum_{\alpha\beta} \sum_{\boldsymbol{k}} \left[ A_{\boldsymbol{k}}^{\alpha\beta} a_{\boldsymbol{k}\alpha}^\dagger a_{\boldsymbol{k}\beta} + A_{-\boldsymbol{k}}^{\beta\alpha} a_{-\boldsymbol{k}\alpha} a_{-\boldsymbol{k}\beta}^\dagger + \left( B_{\boldsymbol{k}}^{\alpha\beta} a_{\boldsymbol{k}\alpha}^\dagger a_{-\boldsymbol{k}\beta}^\dagger + \bar{B}_{\boldsymbol{k}}^{\alpha\beta} a_{-\boldsymbol{k}\beta} a_{\boldsymbol{k}\alpha} \right) \right], \tag{S19a}$$

$$H_3 = \frac{1}{2!} \frac{1}{\sqrt{N_c}} \sum_{\alpha\beta\mu} \sum_{\boldsymbol{k}\boldsymbol{k}'} \left[ T_{\boldsymbol{k}\boldsymbol{k}'}^{\alpha\beta\mu} a_{\boldsymbol{k}\alpha}^\dagger a_{\boldsymbol{k}'\beta}^\dagger a_{\boldsymbol{k}+\boldsymbol{k}',\mu} + \bar{T}_{\boldsymbol{k}\boldsymbol{k}'}^{\alpha\beta\mu} a_{\boldsymbol{k}+\boldsymbol{k}',\mu}^\dagger a_{\boldsymbol{k}'\beta} a_{\boldsymbol{k}\alpha} \right], \tag{S19b}$$

$$H_4 = \frac{1}{N_c} \sum_{\alpha\beta\mu\nu} \sum_{\boldsymbol{k}\boldsymbol{k}'\boldsymbol{q}} \left[ \frac{1}{(2!)^2} V_{\boldsymbol{k}\boldsymbol{k}[\boldsymbol{q}]}^{\alpha\beta\mu\nu} a_{\boldsymbol{k}+\boldsymbol{q},\alpha}^\dagger a_{\boldsymbol{k}'-\boldsymbol{q},\beta}^\dagger a_{\boldsymbol{k}'\mu} a_{\boldsymbol{k}\nu} + \frac{1}{3!} \left( D_{\boldsymbol{k}\boldsymbol{k}'\boldsymbol{q}}^{\alpha\beta\mu\nu} a_{\boldsymbol{k}\alpha}^\dagger a_{\boldsymbol{k}'\beta}^\dagger a_{\boldsymbol{q}\mu}^\dagger a_{\boldsymbol{k}+\boldsymbol{k}'+\boldsymbol{q},\nu} + \text{h.c.} \right) \right]. \tag{S19c}$$

In terms of the local exchange matrices [Eq. (S3)] one can write

$$A_{\boldsymbol{k}}^{\alpha\beta} = \mathcal{J}_{\boldsymbol{k},\alpha\beta}^{+-} - \delta_{\alpha\beta} \sum_{\mu} \mathcal{J}_{\boldsymbol{0},\alpha\mu}^{00}, \tag{S20a}$$

$$B_{\boldsymbol{k}}^{\alpha\beta} = \mathcal{J}_{\boldsymbol{k},\alpha\beta}^{++}, \tag{S20b}$$

$$T_{\boldsymbol{k}\boldsymbol{k}'}^{\alpha\beta\mu} = -\left[ \delta_{\alpha\mu} \mathcal{J}_{\boldsymbol{k}',\beta\alpha}^{+0} + \delta_{\beta\mu} \mathcal{J}_{\boldsymbol{k},\alpha\beta}^{+0} \right], \tag{S20c}$$

$$V_{\boldsymbol{k}\boldsymbol{k}'[\boldsymbol{q}]}^{\alpha\beta\mu\nu} = \left( \delta_{\alpha\mu} \delta_{\beta\nu} \mathcal{J}_{\boldsymbol{k}-\boldsymbol{k}'+\boldsymbol{q},\alpha\beta}^{00} + \delta_{\alpha\nu} \delta_{\beta\mu} \mathcal{J}_{\boldsymbol{q},\alpha\beta}^{00} \right) - \left( \delta_{\mu\nu} \delta_{\mu\beta} \mathcal{J}_{\boldsymbol{k}+\boldsymbol{q},\alpha\nu}^{+-} + \delta_{\alpha\beta} \delta_{\alpha\mu} \mathcal{J}_{\boldsymbol{k},\alpha\nu}^{+-} \right), \tag{S20d}$$

$$D_{\boldsymbol{k}\boldsymbol{k}'\boldsymbol{q}}^{\alpha\beta\mu\nu} = -\frac{3}{4} \left( \delta_{\alpha\mu} \delta_{\alpha\nu} \mathcal{J}_{\boldsymbol{k}',\beta\alpha}^{++} + \delta_{\mu\beta} \delta_{\nu\beta} \mathcal{J}_{\boldsymbol{k},\alpha\beta}^{++} \right), \tag{S20e}$$

where the four-magnon vertices have been left unsymmetrized for brevity.

When $1/S \to 0$, the interactions encoded in $H_3$ and $H_4$ can be included perturbatively since they are $O(S^{-1/2})$ and $O(S^{-1})$ with respect to the linear spin-wave parts. Our main interest is the

(retarded) magnon Green's function, including both normal and anomalous parts. We define the real-frequency retarded Green's functions as

$$G^{R,-+}_{\alpha\alpha'}(\boldsymbol{k},\omega) \equiv -i\int dt e^{i\omega t}\left\{\Theta(t)\left\langle[a_{\boldsymbol{k}\alpha}(t), a^{\dagger}_{\boldsymbol{k}\alpha'}(0)]\right\rangle\right\}, \tag{S21a}$$

$$G^{R,--}_{\alpha\alpha'}(\boldsymbol{k},\omega) \equiv -i\int dt e^{i\omega t}\left\{\Theta(t)\left\langle[a_{\boldsymbol{k}\alpha}(t), a_{-\boldsymbol{k}\alpha'}(0)]\right\rangle\right\}, \tag{S21b}$$

$$G^{R,++}_{\alpha\alpha'}(\boldsymbol{k},\omega) \equiv -i\int dt e^{i\omega t}\left\{\Theta(t)\left\langle[a^{\dagger}_{-\boldsymbol{k}\alpha}(t), a^{\dagger}_{\boldsymbol{k}\alpha'}(0)]\right\rangle\right\}, \tag{S21c}$$

$$G^{R,+-}_{\alpha\alpha'}(\boldsymbol{k},\omega) \equiv -i\int dt e^{i\omega t}\left\{\Theta(t)\left\langle[a^{\dagger}_{-\boldsymbol{k}\alpha}(t), a_{-\boldsymbol{k}\alpha'}(0)]\right\rangle\right\}, \tag{S21d}$$

where $\langle\cdots\rangle$ is a ground state average. These can be organized into a matrix Green's function

$$\boldsymbol{G}^{R}(\boldsymbol{k},\omega) \equiv \begin{pmatrix} \boldsymbol{G}^{R,-+}(\boldsymbol{k},\omega) & \boldsymbol{G}^{R,--}(\boldsymbol{k},\omega) \\ \boldsymbol{G}^{R,++}(\boldsymbol{k},\omega) & \boldsymbol{G}^{R,+-}(\boldsymbol{k},\omega) \end{pmatrix} \equiv \left[\boldsymbol{\sigma}_3(\omega + i0^+) - S\boldsymbol{M}_{\boldsymbol{k}} - \boldsymbol{\Sigma}^{R}(\boldsymbol{k},\omega)\right]^{-1}. \tag{S22}$$

The self-energy, $\boldsymbol{\Sigma}^R(\boldsymbol{k},\omega)$, is generated by interactions, first at $O(S^0)$. As for the Green's function, this contains both normal and anomalous parts. The advanced version of this Green's function can be determined similarly, satisfying the relation $\boldsymbol{G}^A(\boldsymbol{k},\omega) = \boldsymbol{G}^R(\boldsymbol{k},\omega)^{\dagger}$.

The relevant diagrams at $O(S^0)$ in the magnon interactions are given in Fig. 3 of the main text. One involves a single four-magnon interaction, with the remaining two diagrams involving two three-magnon interactions [2]. The first two diagrams, the "droplet" and "tadpole", are static and thus effectively renormalize $\boldsymbol{M}_{\boldsymbol{k}}$. The final "bubble" diagram is dynamic and has non-trivial frequency dependence; when present this can lead to spontaneous decay of the one-magnon excitations into the two-magnon continuum [2].

The (sharp) magnon modes can then be determined from examination of the poles of the magnon Green's function. This amounts to solving the non-linear eigenvalue equation

$$\det\left(\omega + i0^+ - \boldsymbol{\sigma}_3\left[S\boldsymbol{M}_{\boldsymbol{k}} + \boldsymbol{\Sigma}^R(\boldsymbol{k},\omega)\right]\right) = 0, \tag{S23}$$

for the frequency $\omega$. In the limit of $1/S \to 0$, the eigenvalue problem can be solved by treating $\boldsymbol{\Sigma}^R(\boldsymbol{k},\omega)$ as a perturbation to the eigenvalues and eigenvectors of $\boldsymbol{M}_{\boldsymbol{k}}$. Since the self-energy is in general non-Hermitian, these are quasi-normal modes that include both a real and imaginary part, with $\omega \equiv E_{\boldsymbol{k}\alpha} - i\Gamma_{\boldsymbol{k}\alpha}$. Expanding about the energies, $S\epsilon_{\boldsymbol{k}\alpha}$, found at $O(S)$ one finds the effective eigenvalue problem

$$\boldsymbol{\sigma}_3\left[S\boldsymbol{M}_{\boldsymbol{k}} + \boldsymbol{\Sigma}^R(\boldsymbol{k}, S\epsilon_{\boldsymbol{k}\alpha})\right]\boldsymbol{\mathcal{V}}_{\boldsymbol{k}\alpha} = (E_{\boldsymbol{k}\alpha} - i\Gamma_{\boldsymbol{k}\alpha})\boldsymbol{\mathcal{V}}_{\boldsymbol{k}\alpha}, \tag{S24}$$

for each mode found in linear spin-wave theory. If $\epsilon_{\boldsymbol{k}\alpha}$ is non-degenerate (generically) this can be via simple perturbation theory, giving

$$E_{\boldsymbol{k}\alpha} - i\Gamma_{\boldsymbol{k}\alpha} = S\epsilon_{\boldsymbol{k}\alpha} + \boldsymbol{V}^{\dagger}_{\boldsymbol{k}\alpha}\boldsymbol{\sigma}_3\boldsymbol{\Sigma}^R(\boldsymbol{k}, S\epsilon_{\boldsymbol{k}\alpha})\boldsymbol{V}_{\boldsymbol{k}\alpha} + O(S^{-1}). \tag{S25}$$

Similarly $\boldsymbol{\mathcal{V}}_{\boldsymbol{k}\alpha} = \boldsymbol{V}_{\boldsymbol{k}\alpha} + O(S^{-1})$. The eigenvectors analogous to $\boldsymbol{W}_{-\boldsymbol{k}\alpha}$, which we define as $\boldsymbol{\mathcal{W}}_{-\boldsymbol{k},\alpha}$, can be determined in a similar fashion. We note that this perturbative assumption can fail under certain circumstances, even as $1/S \to 0$; see Ref. [2] for details.

### A. Pseudo-Goldstone modes

The pseudo-Goldstone modes we are interested in have two features that distinguish them from the simple case presented above: (i) their energy at $O(S)$ vanishes and (ii) the subspace associated with these eigenvalues is two-dimensional, and so degenerate perturbation theory is generically needed. First, note that since the initial linear spin-wave energy is zero, we evaluate the self-energy at zero-frequency in this calculation. If one expands

$$\boldsymbol{\Sigma}^R(\mathbf{0},\omega) = \boldsymbol{\Sigma}^R(\mathbf{0},0) + \omega\frac{\partial\boldsymbol{\Sigma}^R(\mathbf{0},0)}{\partial\omega} + \cdots, \tag{S26}$$

one sees that the frequency derivative term carries an additional factor of $O(S^{-1})$ relative to the leading term and thus can be dropped. Second, we can ignore the distinction between the retarded and advanced self-energies, taking $\boldsymbol{\Sigma}^R(\mathbf{0},0) \sim \boldsymbol{\Sigma}^A(\mathbf{0},0) \equiv \boldsymbol{\Sigma}_0$. Finding the pseudo-Goldstone energy thus amounts to simply diagonalizing the dispersion and self-energy (at zero wave-vector and frequency) projected into the zero-mode subspace.

We consider the two different types of pseudo-Goldstone mode. For the type II case, the projection of the dispersion part, $\boldsymbol{M}_0$, vanishes and one thus needs to diagonalize only

$$\boldsymbol{\sigma}_3\begin{pmatrix} \boldsymbol{V}_0^\dagger\boldsymbol{\Sigma}_0\boldsymbol{V}_0 & \boldsymbol{V}_0^\dagger\boldsymbol{\Sigma}_0\boldsymbol{W}_0 \\ \boldsymbol{W}_0^\dagger\boldsymbol{\Sigma}_0\boldsymbol{V}_0 & \boldsymbol{W}_0^\dagger\boldsymbol{\Sigma}_0\boldsymbol{W}_0 \end{pmatrix}. \tag{S27}$$

Symmetries of the self-energy tell us that $\boldsymbol{\Sigma}_0 = \boldsymbol{\Sigma}_0^\dagger$ and thus diagonalizing this matrix yields two eigenvalues $\pm\Delta$ with

$$\Delta = \sqrt{\left(\boldsymbol{V}_0^\dagger\boldsymbol{\Sigma}_0\boldsymbol{V}_0\right)^2 - \left|\boldsymbol{W}_0^\dagger\boldsymbol{\Sigma}_0\boldsymbol{W}_0\right|^2} + O(S^{-1}). \tag{S28}$$

We thus see that the type II pseudo-Goldstone gap scales as $O(S^0)$. The type I pseudo-Goldstone mode is different since the projected dispersion matrix is not zero. One finds that

$$\begin{pmatrix} \boldsymbol{V}_0^\dagger\boldsymbol{M}_0\boldsymbol{V}_0 & \boldsymbol{V}_0^\dagger\boldsymbol{M}_0\boldsymbol{W}_0 \\ \boldsymbol{W}_0^\dagger\boldsymbol{M}_0\boldsymbol{V}_0 & \boldsymbol{W}_0^\dagger\boldsymbol{M}_0\boldsymbol{W}_0 \end{pmatrix} = \frac{1}{2\mu}\begin{pmatrix} +1 & +1 \\ +1 & +1 \end{pmatrix}. \tag{S29}$$

One thus must diagonalize

$$\frac{S}{2\mu}\begin{pmatrix} +1 & +1 \\ -1 & -1 \end{pmatrix} + \begin{pmatrix} \boldsymbol{V}_0^\dagger\boldsymbol{\Sigma}_0\boldsymbol{V}_0 & \boldsymbol{V}_0^\dagger\boldsymbol{\Sigma}_0\boldsymbol{W}_0 \\ -\boldsymbol{W}_0^\dagger\boldsymbol{\Sigma}_0\boldsymbol{V}_0 & -\boldsymbol{W}_0^\dagger\boldsymbol{\Sigma}_0\boldsymbol{W}_0 \end{pmatrix}. \tag{S30}$$

Using again that $\boldsymbol{\Sigma}_0$ is Hermitian, as well as the definition of $\mu$ [Eq. (S16)], one finds the pseudo-Goldstone gap

$$\Delta = S^{1/2}\sqrt{2\mathrm{Re}\left[\boldsymbol{V}_0^\dagger\boldsymbol{\Sigma}_0\boldsymbol{\sigma}_3\boldsymbol{M}_0\boldsymbol{V}_0\right]} + O(S^{-1/2}). \tag{S31}$$

This scales as $S^{1/2}$, distinct from that found in the type II case.

More practically, the computation of $\boldsymbol{\Sigma}_0$ requires the evaluation of sums that involve the eigenvectors and eigenvalues of $\boldsymbol{\sigma}_3\boldsymbol{M}_{\boldsymbol{k}}$. Due to the presence of the zero-modes, these are somewhat

ill-defined. To circumvent this, we include a small, but finite, chemical potential for the magnons $\sim \mu \sum_{\boldsymbol{k}\alpha} a^{\dagger}_{\boldsymbol{k}\alpha} a_{\boldsymbol{k}\alpha}$, which plays the role of a physical pinning field. This resolves any singularities and renders the sums well-defined. To recover the thermodynamic limit, one first takes the system size to be large ($L \to \infty$) before removing the regulator ($\mu \to 0$). Note that the inclusion of $\mu$, absent true Goldstone modes, directly implies that $\boldsymbol{\Sigma}^R(\boldsymbol{0}, 0) = \boldsymbol{\Sigma}^A(\boldsymbol{0}, 0)$, since the two-magnon continuum then starts at $2\mu$. For most cases of interest the pseudo-Goldstone gap depends only weakly on the pinning field and thus the above procedure, while strictly required, is mostly unnecessary. An alternative regulator is to use of modified boundary conditions (e.g. anti-periodic) to remove the zero mode; these have the advantage of only having a single limit to evaluate ($L \to \infty$), but the disadvantage that they may break some symmetries of the original problem.

## S3. PROOF OF CURVATURE FORMULA

We now show how the gap computed from non-linear spin-wave theory can be directly related to the curvatures of the classical and quantum parts of the spin-wave energies computed in linear spin-wave theory. The strategy we take is based on the "self-correcting" nature of the spin-wave expansion: if one performs the Holstein-Primakoff expansion about a classical ground state sufficiently close to the true ground state, one should recover the true ground state properties, order by order in $1/S$. This then implies that there is some degree of independence with respect to the initial classical starting point.

We show this in a few stages: first we will give an explicit demonstration of this "self-correction" at the level of linear spin-wave theory. At higher order we proceed more implicitly, showing that the same physics is encoded in a sum rule for the spectral function. Using this sum rule will show that the curvature formula discussed in the main text holds. As a warm up we do this for gapped modes in linear spin-wave theory, before proceeding to the type I and type II pseudo-Goldstone modes of interest.

### A. Self-correcting linear spin-waves

Before delving into the main proof, we first show how this self-correcting behavior appears in practice. Consider the linear spin-wave theory discussed previously [Eq. (S4)], but expanded about a state which is *not* the classical ground state. In this case one finds additional terms in the Hamiltonian that are linear in the magnons.

We consider expanding about states that are related to the ground state by small rotations about the local $\hat{\boldsymbol{x}}_\alpha$ and $\hat{\boldsymbol{y}}_\alpha$ directions. We will assume these deformations describe the degrees of freedom involved in the low-lying, long-wavelength spin-waves of the problem. Explicitly, if $\hat{\boldsymbol{e}}_{\alpha,0}$ and $\hat{\boldsymbol{e}}_{\alpha,\pm}$

define the local frames for the classical ground state, then we define

$$\hat{\boldsymbol{e}}_{\alpha,+}(\zeta) \equiv (1 - |\zeta|^2)\hat{\boldsymbol{e}}_{\alpha,+} - \zeta\hat{\boldsymbol{e}}_{\alpha,0} - \zeta^2\hat{\boldsymbol{e}}_{\alpha,-} + O(\zeta^3), \tag{S32a}$$

$$\hat{\boldsymbol{e}}_{\alpha,0}(\zeta) \equiv (1 - |\zeta|^2)\hat{\boldsymbol{e}}_{\alpha,0} + \bar{\zeta}\hat{\boldsymbol{e}}_{\alpha,+} + \zeta\hat{\boldsymbol{e}}_{\alpha,-} + O(\zeta^3), \tag{S32b}$$

$$\hat{\boldsymbol{e}}_{\alpha,-}(\zeta) \equiv (1 - |\zeta|^2)\hat{\boldsymbol{e}}_{\alpha,-} - \bar{\zeta}\hat{\boldsymbol{e}}_{\alpha,0} - \bar{\zeta}^2\hat{\boldsymbol{e}}_{\alpha,+} + O(\zeta^3), \tag{S32c}$$

where the complex variable $\zeta \equiv (\phi + i\theta)/\sqrt{2}$ encodes both rotations and $|\zeta| \ll 1$.

Performing the Holstein-Primakoff expansion one then finds the Hamiltonian

$$H(\zeta) = S(S+1)N\epsilon_{\rm cl}(\zeta) + SH_2(\zeta) + S^{3/2}H_1(\zeta) + O(S^{1/2}). \tag{S33}$$

The quadratic part we have encountered previously [Eq. (S4)], with

$$H_2(\zeta) \equiv \frac{1}{2}\sum_{\boldsymbol{k}} \begin{pmatrix} [\boldsymbol{a}^\dagger_{\boldsymbol{k}}]^\intercal & \boldsymbol{a}^\intercal_{-\boldsymbol{k}} \end{pmatrix} \begin{pmatrix} \boldsymbol{A}_{\boldsymbol{k}}(\zeta) & \boldsymbol{B}_{\boldsymbol{k}}(\zeta) \\ \boldsymbol{B}^\dagger_{\boldsymbol{k}}(\zeta) & \boldsymbol{A}^\intercal_{-\boldsymbol{k}}(\zeta) \end{pmatrix} \begin{pmatrix} \boldsymbol{a}_{\boldsymbol{k}} \\ \boldsymbol{a}^\dagger_{-\boldsymbol{k}} \end{pmatrix}. \tag{S34}$$

The linear part appears as

$$H_1(\zeta) = \sum_\alpha \left[\lambda_\alpha(\zeta)a^\dagger_{\boldsymbol{0},\alpha} + \bar{\lambda}_\alpha(\zeta)a_{\boldsymbol{0},\alpha}\right] = \begin{pmatrix} \boldsymbol{\lambda}(\zeta)^\dagger & \boldsymbol{\lambda}(\zeta)^\intercal \end{pmatrix} \begin{pmatrix} \boldsymbol{a}_{\boldsymbol{0}} \\ \boldsymbol{a}^\dagger_{\boldsymbol{0}} \end{pmatrix}, \tag{S35}$$

where we have defined

$$\begin{pmatrix} \boldsymbol{\lambda}(\zeta) \\ \boldsymbol{\lambda}(\zeta)^\dagger \end{pmatrix} = N^{1/2}\boldsymbol{M}_0 \begin{pmatrix} \zeta\hat{\boldsymbol{u}} \\ \bar{\zeta}\hat{\boldsymbol{u}} \end{pmatrix}, \tag{S36}$$

where the vector $\hat{\boldsymbol{u}}$ is uniform over the sublattices, with $\hat{u}_\alpha \equiv 1/\sqrt{N_s}$.

Our statement of self-correction is then that the ground state energy must be independent of $\phi$ and $\theta$ order by order in $1/S$. At first this appears somewhat contradictory: the constant classical part depends on $\phi$ and $\theta$ and is $O(S^2)$; how can terms at $O(S)$ and $O(S^{3/2})$ cancel it? We can see how this works out directly by shifting the bosons to remove the linear term. Define the shifted boson operators

$$\begin{pmatrix} \boldsymbol{a}_{\boldsymbol{0}} \\ \boldsymbol{a}^\dagger_{\boldsymbol{0}} \end{pmatrix} = \begin{pmatrix} \boldsymbol{b}_{\boldsymbol{0}} \\ \boldsymbol{b}^\dagger_{\boldsymbol{0}} \end{pmatrix} - S^{1/2}\boldsymbol{M}(\zeta)^{-1} \begin{pmatrix} \boldsymbol{\lambda}(\zeta) \\ \boldsymbol{\lambda}(\zeta)^\dagger \end{pmatrix}. \tag{S37}$$

In terms of these shifted bosons, the Hamiltonian is then

$$S(S+1)N\epsilon_{\rm cl}(\zeta) + \frac{S}{2}\sum_{\boldsymbol{k}} \begin{pmatrix} [\boldsymbol{b}^\dagger_{\boldsymbol{k}}]^\intercal & \boldsymbol{b}^\intercal_{-\boldsymbol{k}} \end{pmatrix} \begin{pmatrix} \boldsymbol{A}_{\boldsymbol{k}}(\zeta) & \boldsymbol{B}_{\boldsymbol{k}}(\zeta) \\ \boldsymbol{B}^\dagger_{\boldsymbol{k}}(\zeta) & \boldsymbol{A}^\intercal_{-\boldsymbol{k}}(\zeta) \end{pmatrix} \begin{pmatrix} \boldsymbol{b}_{\boldsymbol{k}} \\ \boldsymbol{b}^\dagger_{-\boldsymbol{k}} \end{pmatrix} - \frac{S^2}{2} \begin{pmatrix} \boldsymbol{\lambda}(\zeta)^\dagger & \boldsymbol{\lambda}(\zeta)^\intercal \end{pmatrix} \boldsymbol{M}(\zeta)^{-1} \begin{pmatrix} \boldsymbol{\lambda}(\zeta) \\ \boldsymbol{\lambda}(\zeta)^\dagger \end{pmatrix}.$$

Since the rotation is only evaluated to $O(\zeta^2)$ we should also expand

$$\epsilon_{\rm cl}(\zeta) = \epsilon_{\rm cl}(0) + \frac{1}{2}\left[\left(\frac{\partial^2\epsilon_{\rm cl}}{\partial\theta^2}\right)_0 \theta^2 + \left(\frac{\partial^2\epsilon_{\rm cl}}{\partial\phi^2}\right)_0 \phi^2 + 2\left(\frac{\partial^2\epsilon_{\rm cl}}{\partial\theta\partial\phi}\right)_0 \theta\phi\right] + O(\zeta^3). \tag{S38}$$

We thus see that the $O(S^2)$ contribution to the energy, to quadratic order in $\zeta$, is then given by

$$S^2N\left\{\epsilon_{\rm cl}(0) + \frac{1}{2}\left[\left(\frac{\partial^2\epsilon_{\rm cl}}{\partial\theta^2}\right)_0 \theta^2 + \left(\frac{\partial^2\epsilon_{\rm cl}}{\partial\phi^2}\right)_0 \phi^2 + 2\left(\frac{\partial^2\epsilon_{\rm cl}}{\partial\theta\partial\phi}\right)_0 \theta\phi\right] - \frac{1}{2}\begin{pmatrix} \bar{\zeta}\hat{\boldsymbol{u}}^\intercal & \zeta\hat{\boldsymbol{u}}^\intercal \end{pmatrix} \boldsymbol{M}_0 \begin{pmatrix} \zeta\hat{\boldsymbol{u}} \\ \bar{\zeta}\hat{\boldsymbol{u}} \end{pmatrix}\right\}. \tag{S39}$$

To connect with the notation for the zero modes, as well as some notation we will introduce later, define

$$\boldsymbol{U}_{\Phi} = \frac{1}{\sqrt{2}}\begin{pmatrix} \hat{\boldsymbol{u}} \\ \hat{\boldsymbol{u}} \end{pmatrix}, \qquad \boldsymbol{U}_{\Theta} = \frac{i}{\sqrt{2}}\begin{pmatrix} \hat{\boldsymbol{u}} \\ -\hat{\boldsymbol{u}} \end{pmatrix}. \tag{S40}$$

One then sees that the shift induced part of the $O(S^2)$ contributions are given as a matrix element of the vector $\phi\boldsymbol{U}_{\Phi} + \theta\boldsymbol{U}_{\Theta}$. For the $O(S^2)$ part of the energy to be independent of $\phi$ and $\theta$, one then must require

$$\left(\frac{\partial^2\epsilon_{\rm cl}}{\partial\phi^2}\right)_0 = \boldsymbol{U}_{\Phi}^{\dagger}\boldsymbol{M}_0\boldsymbol{U}_{\Phi}, \qquad \left(\frac{\partial^2\epsilon_{\rm cl}}{\partial\theta\partial\phi}\right)_0 = \boldsymbol{U}_{\Theta}^{\dagger}\boldsymbol{M}_0\boldsymbol{U}_{\Phi}, \qquad \left(\frac{\partial^2\epsilon_{\rm cl}}{\partial\theta^2}\right)_0 = \boldsymbol{U}_{\Theta}^{\dagger}\boldsymbol{M}_0\boldsymbol{U}_{\Theta}. \tag{S41}$$

This can be related to the energy of the spin-wave mode in the subspace spanned by these two vectors. Note that

$$\boldsymbol{U}_{\Phi}^{\dagger}\boldsymbol{\sigma}_3\boldsymbol{U}_{\Phi} = \boldsymbol{U}_{\Theta}^{\dagger}\boldsymbol{\sigma}_3\boldsymbol{U}_{\Theta} = 0, \qquad \boldsymbol{U}_{\Phi}^{\dagger}\boldsymbol{\sigma}_3\boldsymbol{U}_{\Theta} = +i. \tag{S42}$$

Projecting the eigenvalue equation for the zone center spin-wave into this subspace then yields the two by two problem

$$\det\left[S\begin{pmatrix} \boldsymbol{U}_{\Phi}^{\dagger}\boldsymbol{M}_0\boldsymbol{U}_{\Phi} & \boldsymbol{U}_{\Phi}^{\dagger}\boldsymbol{M}_0\boldsymbol{U}_{\Theta} \\ \boldsymbol{U}_{\Theta}^{\dagger}\boldsymbol{M}_0\boldsymbol{U}_{\Phi} & \boldsymbol{U}_{\Theta}^{\dagger}\boldsymbol{M}_0\boldsymbol{U}_{\Theta} \end{pmatrix} - \omega\begin{pmatrix} 0 & -i \\ +i & 0 \end{pmatrix}\right] = 0. \tag{S43}$$

There are two solutions, $\pm\epsilon_0$, where

$$\epsilon_0 = S\sqrt{(\boldsymbol{U}_{\Phi}^{\dagger}\boldsymbol{M}_0\boldsymbol{U}_{\Phi})(\boldsymbol{U}_{\Theta}^{\dagger}\boldsymbol{M}_0\boldsymbol{U}_{\Theta}) - |\boldsymbol{U}_{\Theta}^{\dagger}\boldsymbol{M}_0\boldsymbol{U}_{\Phi}|^2}, \tag{S44}$$

where we used that $\boldsymbol{U}_{\Theta}^{\dagger}\boldsymbol{M}_0\boldsymbol{U}_{\Phi} = \boldsymbol{U}_{\Phi}^{\dagger}\boldsymbol{M}_0\boldsymbol{U}_{\Theta}$. The energy of this mode is then directly related to the curvatures, with Eq. (S41) and Eq. (S44) implying that

$$\epsilon_0 = S\sqrt{\left(\frac{\partial^2\epsilon_{\rm cl}}{\partial\theta^2}\right)_0\left(\frac{\partial^2\epsilon_{\rm cl}}{\partial\phi^2}\right)_0 - \left(\frac{\partial^2\epsilon_{\rm cl}}{\partial\theta\partial\phi}\right)_0^2}. \tag{S45}$$

Alternatively, this relation can be worked explicitly by expressing the curvatures and $\epsilon_0$ directly in terms of the relevant exchange matrices.

We have thus seen that enforcing the condition that the ground state energy is independent of the initial state at $O(S^2)$, we have found a relation between a spin-wave energy computed at $O(S)$ and curvatures of the classical energies, computed at $O(S^2)$. Our goal in the next few sections is to establish the same kind of relation, but between a spin-wave energy at $O(S^0)$ or $O(S^{1/2})$ and the curvatures of the classical and quantum energies at $O(S^2)$ and $O(S)$. Since we will not be able to solve the theory explicitly at $O(S^0)$, as we did at $O(S)$ above, our methods will have to be somewhat more indirect. However the essence of the argument remains the same.

### B. First moment sum rule and spectral functions

To attack this problem for interacting spin-waves, we will first define a rotated Hamiltonian that will serve as the starting point of the Holstein-Primakoff expansion. Since we want to leverage an exact sum rule, we will do this at the level of spin operators, rather than Holstein-Primakoff bosons (as was done in Sec. S3 A).

To motivate this, define the explicit zero-mode magnons [1]

$$\gamma_0 = \sum_\alpha \left[\bar{X}_0^\alpha a_{\mathbf{0},\alpha} - \bar{Y}_0^\alpha a_{\mathbf{0},\alpha}^\dagger\right] = \boldsymbol{V}_0^\dagger \boldsymbol{\sigma}_3 \begin{pmatrix} \boldsymbol{a}_\mathbf{0} \\ \boldsymbol{a}_\mathbf{0}^\dagger \end{pmatrix} = -\left( [\boldsymbol{a}_\mathbf{0}^\dagger]^\intercal \boldsymbol{a}_\mathbf{0}^\intercal \right) \boldsymbol{\sigma}_3 \boldsymbol{W}_0, \tag{S46a}$$

$$\gamma_0^\dagger = \sum_\alpha \left[X_0^\alpha a_{\mathbf{0},\alpha}^\dagger - Y_0^\alpha a_{\mathbf{0},\alpha}\right] = -\boldsymbol{W}_0^\dagger \boldsymbol{\sigma}_3 \begin{pmatrix} \boldsymbol{a}_\mathbf{0} \\ \boldsymbol{a}_\mathbf{0}^\dagger \end{pmatrix} = \left( [\boldsymbol{a}_\mathbf{0}^\dagger]^\intercal \boldsymbol{a}_\mathbf{0}^\intercal \right) \boldsymbol{\sigma}_3 \boldsymbol{V}_0. \tag{S46b}$$

By combining these, we can create a pair of Hermitian operators that can be defined directly in terms of the spins. We define a position-like operator, $\Phi$, and momentum-like operator, $\Theta$, as

$$\Phi \equiv \sum_{\boldsymbol{r}\alpha} [(\mathrm{Re}X_0^\alpha - \mathrm{Re}Y_0^\alpha)\, S_{\boldsymbol{r}\alpha}^x + (\mathrm{Im}X_0^\alpha + \mathrm{Im}Y_0^\alpha)\, S_{\boldsymbol{r}\alpha}^y] = \sqrt{\frac{SN}{2}} \left[\gamma_0^\dagger + \gamma_0\right] + O(S^{-1/2}), \tag{S47a}$$

$$\Theta \equiv \sum_{\boldsymbol{r}\alpha} [-(\mathrm{Im}X_0^\alpha - \mathrm{Im}Y_0^\alpha)\, S_{\boldsymbol{r}\alpha}^x + (\mathrm{Re}X_0^\alpha + \mathrm{Re}Y_0^\alpha)\, S_{\boldsymbol{r}\alpha}^y] = i\sqrt{\frac{SN}{2}} \left[\gamma_0^\dagger - \gamma_0\right] + O(S^{-1/2}), \tag{S47b}$$

which satisfy $[\Phi, \Theta] = iNS$ at leading order in $1/S$ and map to combinations of the zero-mode magnons. These operators represent the general form of the soft directions discussed in the main text; given a spin model, the appropriate semi-classical variables can thus be obtained from the vectors that characterize the zero mode in linear spin-wave theory, via Eq. (S47).

Using these two operators, $\Phi$ and $\Theta$, we define the local spin rotation

$$U(\phi, \theta) \equiv e^{-i\phi\Phi} e^{-i\theta\Theta} = e^{-i\theta\Theta} e^{-i\phi\Phi} e^{-i\theta\phi NS}. \tag{S48}$$

Note that since $[\Phi, \Theta]$ is a constant, the order of operations is unimportant at leading order in $1/S$. This can be used to define the transformed Hamiltonian $\mathcal{H}(\phi, \theta) \equiv U(\phi, \theta)^\dagger H U(\phi, \theta)$ where $\mathcal{H}(0, 0) = H$. The Hamiltonian can be expanded as

$$\begin{aligned} \mathcal{H}(\phi, \theta) &\sim e^{i\theta\Theta} \left( H + i\phi[\Phi, H] - \frac{\phi^2}{2}[\Phi, [\Phi, H]] + \cdots \right) e^{-i\theta\Theta}, \\ &\sim H + i\left(\theta[\Theta, H] + \phi[\Phi, H]\right) - \frac{1}{2}\left(\phi^2[\Phi, [\Phi, H]] + 2\phi\theta[\Phi, [\Theta, H]] + \theta^2[\Theta, [\Theta, H]]\right). \end{aligned}$$

We thus can write the derivatives

$$\begin{aligned} \left(\frac{\partial^2 \mathcal{H}}{\partial \phi^2}\right)_0 &= -[\Phi, [\Phi, H]], & \left(\frac{\partial^2 \mathcal{H}}{\partial \phi \partial \theta}\right)_0 &= -[\Phi, [\Theta, H]], \\ \left(\frac{\partial^2 \mathcal{H}}{\partial \theta \partial \phi}\right)_0 &= -[\Theta, [\Phi, H]], & \left(\frac{\partial^2 \mathcal{H}}{\partial \theta^2}\right)_0 &= -[\Theta, [\Theta, H]]. \end{aligned} \tag{S49}$$

Now while the Hamiltonian is not invariant under this transformation, the ground state energy is trivially invariant under this operation.

If we thus define the ground state energy of $\mathcal{H}(\phi,\theta)$ to be $E(\phi,\theta)$, then one has $E(\phi,\theta) = E(0,0)$ identically, implying that all derivatives with respect to $\phi$ and $\theta$ vanish. The vanishing of these derivatives has implications for the correlation functions and expectation values of $\Phi$ and $\Theta$. For example, the vanishing of the first derivatives implies the (trivial) statement that $\langle[\Phi, H]\rangle = \langle[\Theta, H]\rangle = 0$, where $\langle\cdots\rangle$ is a ground state average with respect to $H$. The implications from the second derivative are less trivial, and imply sum rules for the spectral function of these operators.

First recall the definition of the spectral function of a pair of operators $O$ and $O'$

$$A_{OO'}(\Omega) \equiv \frac{1}{2i}\left[G^R_{OO'}(\Omega) - G^A_{OO'}(\Omega)\right], \tag{S50}$$

where $G^R_{OO'}(\omega)$ and $G^A_{OO'}(\omega)$ are the associated retarded and advanced Green's functions for these operators. The vanishing of the second derivatives then implies the sum rules

$$\begin{aligned}\int d\Omega\,\Omega\,A_{\Phi\Phi}(\Omega) &= \left\langle\left(\frac{\partial^2\mathcal{H}}{\partial\phi^2}\right)_0\right\rangle, & \int d\Omega\,\Omega\,A_{\Phi\Theta}(\Omega) &= \left\langle\left(\frac{\partial^2\mathcal{H}}{\partial\phi\partial\theta}\right)_0\right\rangle,\\ \int d\Omega\,\Omega\,A_{\Theta\Phi}(\Omega) &= \left\langle\left(\frac{\partial^2\mathcal{H}}{\partial\theta\partial\phi}\right)_0\right\rangle, & \int d\Omega\,\Omega\,A_{\Theta\Theta}(\Omega) &= \left\langle\left(\frac{\partial^2\mathcal{H}}{\partial\theta^2}\right)_0\right\rangle.\end{aligned} \tag{S51}$$

We refer to these collectively as the *first moment sum rule*. We stress that the expectation value, $\langle\cdots\rangle$, is with respect to the ground state of $H$, not the ground state of $\mathcal{H}(\theta,\phi)$. Alternatively, these relations are a special case of more general expressions for the moments of the spectral function [3, 4] or can be seen as a generalized version of the $f$-sum rule.

These spectral functions can be related to the spectral function of the magnon operators. From Eq. (S47), we express these as

$$A_{\Phi\Phi}(\Omega) = \frac{SN}{2}\left[A_{\gamma_0^\dagger,\gamma_0}(\Omega) + A_{\gamma_0,\gamma_0^\dagger}(\Omega) + A_{\gamma_0^\dagger,\gamma_0^\dagger}(\Omega) + A_{\gamma_0,\gamma_0}(\Omega)\right] + O(S^{-1/2}), \tag{S52a}$$

$$A_{\Phi\Theta}(\Omega) = \frac{iSN}{2}\left[A_{\gamma_0,\gamma_0^\dagger}(\Omega) - A_{\gamma_0^\dagger,\gamma_0}(\Omega) + A_{\gamma_0^\dagger,\gamma_0^\dagger}(\Omega) - A_{\gamma_0,\gamma_0}(\Omega)\right] + O(S^{-1/2}), \tag{S52b}$$

$$A_{\Theta\Phi}(\Omega) = \frac{iSN}{2}\left[A_{\gamma_0^\dagger,\gamma_0}(\Omega) - A_{\gamma_0,\gamma_0^\dagger}(\Omega) + A_{\gamma_0^\dagger,\gamma_0^\dagger}(\Omega) - A_{\gamma_0,\gamma_0}(\Omega)\right] + O(S^{-1/2}), \tag{S52c}$$

$$A_{\Theta\Theta}(\Omega) = \frac{SN}{2}\left[A_{\gamma_0^\dagger,\gamma_0}(\Omega) + A_{\gamma_0,\gamma_0^\dagger}(\Omega) - A_{\gamma_0^\dagger,\gamma_0^\dagger}(\Omega) - A_{\gamma_0,\gamma_0}(\Omega)\right] + O(S^{-1/2}). \tag{S52d}$$

Its useful to relate this back to the Green's functions we have define for the magnons. Using the retarded and advanced magnon Green's functions [Eq. (S22)] we can define the magnon spectral function

$$\boldsymbol{A}(\boldsymbol{k},\Omega) \equiv \frac{1}{2i}\left[\boldsymbol{G}^R(\boldsymbol{k},\Omega) - \boldsymbol{G}^A(\boldsymbol{k},\Omega)\right]. \tag{S53}$$

Then each of these pieces can be expressed in terms of the one-magnon spectral function via

$$\begin{aligned}A_{\gamma_0,\gamma_0^\dagger}(\Omega) &= +\boldsymbol{V}_0^\dagger\boldsymbol{\sigma}_3\boldsymbol{A}(\boldsymbol{0},\Omega)\boldsymbol{\sigma}_3\boldsymbol{V}_0, & A_{\gamma_0,\gamma_0}(\Omega) &= -\boldsymbol{V}_0^\dagger\boldsymbol{\sigma}_3\boldsymbol{A}(\boldsymbol{0},\Omega)\boldsymbol{\sigma}_3\boldsymbol{W}_0,\\ A_{\gamma_0^\dagger,\gamma_0^\dagger}(\Omega) &= -\boldsymbol{W}_0^\dagger\boldsymbol{\sigma}_3\boldsymbol{A}(\boldsymbol{0},\Omega)\boldsymbol{\sigma}_3\boldsymbol{V}_0, & A_{\gamma_0^\dagger,\gamma_0}(\Omega) &= +\boldsymbol{W}_0^\dagger\boldsymbol{\sigma}_3\boldsymbol{A}(\boldsymbol{0},\Omega)\boldsymbol{\sigma}_3\boldsymbol{W}_0.\end{aligned} \tag{S54}$$

This can be made cleaner via the definition of some rotated basis vectors for the zero-mode subspace; define

$$\boldsymbol{U}_\Theta = \frac{\boldsymbol{V}_0 + \boldsymbol{W}_0}{\sqrt{2}}, \qquad \boldsymbol{U}_\Phi = \frac{\boldsymbol{V}_0 - \boldsymbol{W}_0}{i\sqrt{2}}. \tag{S55}$$

From the normalization conditions on $\boldsymbol{V}_0$ and $\boldsymbol{W}_0$ [Eq. (S9)] one has that

$$\boldsymbol{U}_\Phi^\dagger \boldsymbol{\sigma}_3 \boldsymbol{U}_\Phi = \boldsymbol{U}_\Theta^\dagger \boldsymbol{\sigma}_3 \boldsymbol{U}_\Theta = 0, \qquad \boldsymbol{U}_\Phi^\dagger \boldsymbol{\sigma}_3 \boldsymbol{U}_\Theta = +i. \tag{S56}$$

The set of spectral functions can be expressed compactly if if we define an index $\mu, \nu = \Phi$ or $\Theta$, we can write

$$A_{\mu\nu}(\Omega) = SN\boldsymbol{U}_\mu^\dagger \left[\boldsymbol{\sigma}_3 \boldsymbol{A}(\boldsymbol{0},\Omega)\boldsymbol{\sigma}_3\right] \boldsymbol{U}_\nu. \tag{S57}$$

Coming back to the first moment sum rule, we then have that

$$\boldsymbol{U}_\mu^\dagger \boldsymbol{\sigma}_3 \left[\int d\Omega\, \Omega\, \boldsymbol{A}(\boldsymbol{0},\Omega)\right] \boldsymbol{\sigma}_3 \boldsymbol{U}_\nu = \frac{1}{SN}\left\langle \left(\frac{\partial^2 \mathcal{H}}{\partial\lambda_\mu \partial\lambda_\nu}\right)_0 \right\rangle, \tag{S58}$$

where $\lambda_\Phi = \phi$ and $\lambda_\Theta = \theta$. This is the key result that will allow us to establish the equivalence statement.

### C. Warm up: No pseudo-Goldstone mode

As an example consider the non-interacting case where there is no accidental degeneracy and no zero mode. If one performs a spin-wave expansion of $\mathcal{H}(\phi,\theta)$ then one will find an $O(S^2)$ classical contribution to the energy given as

$$\mathcal{H}(\phi,\theta) = S^2 N \epsilon_{\rm cl}(\phi,\theta) + O(S), \tag{S59}$$

where $\epsilon_{\rm cl}(\phi,\theta)$ is the classical energy density in the rotated configuration. The right hand side of the sum rule [Eq. (S58)] then reads

$$\frac{1}{SN}\left\langle \left(\frac{\partial^2 \mathcal{H}}{\partial\lambda_\mu \partial\lambda_\nu}\right)_0 \right\rangle = S\left(\frac{\partial^2 \epsilon_{\rm cl}}{\partial\lambda_\mu \partial\lambda_\nu}\right)_0 + O(S^0). \tag{S60}$$

For the left side of the sum rule, we consider the magnon spectral function at $O(S)$. In terms of the appropriate eigenvectors and eigenvalues of $\boldsymbol{\sigma}_3 \boldsymbol{M}_0$ one has

$$\boldsymbol{A}(\boldsymbol{0},\omega) = \sum_\alpha \left[\delta(\omega - \epsilon_{\boldsymbol{0},\alpha})\boldsymbol{V}_{\boldsymbol{0},\alpha}\boldsymbol{V}_{\boldsymbol{0},\alpha}^\dagger - \delta(\omega + \epsilon_{\boldsymbol{0},\alpha})\boldsymbol{W}_{\boldsymbol{0},\alpha}\boldsymbol{W}_{\boldsymbol{0},\alpha}^\dagger\right]. \tag{S61}$$

The first moment is then given by

$$\int d\omega\, \omega\, \boldsymbol{A}(\boldsymbol{0},\omega) = \sum_\alpha \epsilon_{\boldsymbol{0},\alpha}\left[\boldsymbol{V}_{\boldsymbol{0},\alpha}\boldsymbol{V}_{\boldsymbol{0},\alpha}^\dagger + \boldsymbol{W}_{\boldsymbol{0},\alpha}\boldsymbol{W}_{\boldsymbol{0},\alpha}^\dagger\right] = \boldsymbol{\sigma}_3 \boldsymbol{M}_0 \boldsymbol{\sigma}_3, \tag{S62}$$

where we have used the spectral decomposition of $\boldsymbol{M}_0$ [1]. Putting these two together one finds that

$$\boldsymbol{U}_\mu^\dagger \boldsymbol{M}_0 \boldsymbol{U}_\nu = S\left(\frac{\partial^2 \epsilon_{\rm cl}}{\partial\lambda_\mu \partial\lambda_\nu}\right)_0. \tag{S63}$$

We thus see that the energies of the spin-wave modes at $O(S)$ in the subspace spanned by $\boldsymbol{U}_\Theta$, $\boldsymbol{U}_\Phi$ can be determined from the curvatures of the classical energy, just as in Sec. S3 A.

### D. Type II pseudo-Goldstone mode

We now consider a case with a type II pseudo-Goldstone mode, as this is a bit simpler than the type I case. Due to the presence of the accidental degeneracy, the spin-wave expansion is stable to $O(S)$ for any choice of $\theta$ and $\phi$. Consider the rotated Hamiltonian

$$\mathcal{H}(\phi,\theta) = \frac{1}{2}\sum_{\boldsymbol{r}\boldsymbol{r}'}\sum_{\alpha\alpha'} \boldsymbol{S}^{\intercal}_{\boldsymbol{r}\alpha}\left[\boldsymbol{R}^{\intercal}_{\alpha}(\phi,\theta)\boldsymbol{J}_{\boldsymbol{r}-\boldsymbol{r}',\alpha\alpha'}\boldsymbol{R}_{\alpha'}(\phi,\theta)\right]\boldsymbol{S}_{\boldsymbol{r}'\alpha'}, \tag{S64}$$

where $\boldsymbol{R}_\alpha(\phi,\theta)$ is the local rotation matrix associated with the operator $U(\phi,\theta)$. Explicitly, the generators of the rotation (i.e. the axis and angle) can be read directly from Eq. (S47). We perform our Holstein-Primakoff expansion about the ground state of $\phi = \theta = 0$ problem which, given we have rotated exchanges, is equivalent to performing the expansion about the state with finite $\phi$ and $\theta$. Since the classical ground state is stable for arbitrary $\phi$ and $\theta$, we can write

$$\mathcal{H}(\phi,\theta) = S(S+1)N\epsilon_{\rm cl}(0,0) + SN\epsilon_{\rm qu}(\phi,\theta) + S\sum_{\boldsymbol{k}\alpha}\epsilon_{\boldsymbol{k}\alpha}(\phi,\theta)\gamma^{\dagger}_{\boldsymbol{k}\alpha}\gamma_{\boldsymbol{k}\alpha} + O(S^{1/2}), \tag{S65}$$

where we have noted that $\epsilon_{\rm cl}(\phi,\theta) = \epsilon_{\rm cl}(0,0)$. The second derivative is then

$$\frac{1}{SN}\left\langle\left(\frac{\partial^2\mathcal{H}}{\partial\lambda_\mu\partial\lambda_\nu}\right)_0\right\rangle = \left(\frac{\partial^2\epsilon_{\rm qu}}{\partial\lambda_\mu\partial\lambda_\nu}\right)_0 + \frac{1}{N}\sum_{\boldsymbol{k}\alpha}\left(\frac{\partial^2\epsilon_{\boldsymbol{k}\alpha}}{\partial\lambda_\mu\partial\lambda_\nu}\right)_0\langle\gamma^{\dagger}_{\boldsymbol{k}\alpha}\gamma_{\boldsymbol{k}\alpha}\rangle + O(S^{-1}). \tag{S66}$$

The magnon expectation value is with respect to the $\phi = \theta = 0$ ground state, and thus is zero in linear spin-wave theory. We can thus say that $\langle\gamma^{\dagger}_{\boldsymbol{k}\alpha}\gamma_{\boldsymbol{k}\alpha}\rangle \sim O(S^{-1})$, and since $\epsilon_{\boldsymbol{k}\alpha}(\phi,\theta) \sim O(S^0)$, these terms are unimportant. The right hand side of the sum rule is then simply given by the curvature of the quantum zero-point energy density

$$\frac{1}{SN}\left\langle\left(\frac{\partial^2\mathcal{H}}{\partial\lambda_\mu\partial\lambda_\nu}\right)_0\right\rangle = \left(\frac{\partial^2\epsilon_{\rm qu}}{\partial\lambda_\mu\partial\lambda_\nu}\right)_0 + O(S^{-1}). \tag{S67}$$

Consider now the left-hand side of the sum rule. Since the right-hand side has a leading contribution of $O(S^0)$, we must also identify such a contribution at this order from the first moment of the spectral function. As discussed in Sec. S2, at $O(S^0)$ the spin-wave energies can be determined by perturbatively including the $O(S^{1/2})$ and $O(S^0)$ interaction terms from the Holstein-Primakoff expansion. This produces a spectral function of the form

$$\boldsymbol{A}(\boldsymbol{0},\omega) = \sum_{\alpha}\left[\mathscr{L}(\omega - E_{\boldsymbol{0},\alpha},\Gamma_{\boldsymbol{0},\alpha})\boldsymbol{\mathcal{V}}_{\boldsymbol{0},\alpha}\boldsymbol{\mathcal{V}}^{\dagger}_{\boldsymbol{0},\alpha} - \mathscr{L}(\omega + E_{\boldsymbol{0},\alpha},\Gamma_{\boldsymbol{0},\alpha})\boldsymbol{\mathcal{W}}_{\boldsymbol{0},\alpha}\boldsymbol{\mathcal{W}}^{\dagger}_{\boldsymbol{0},\alpha}\right], \tag{S68}$$

where the notation for the quasi-normal modes is defined in Sec. S2 and we have defined $\mathcal{L}(\omega,\gamma)$ to be a Lorentzian centered at zero-energy with width $\gamma$, that is

$$\mathscr{L}(\omega,\gamma) \equiv \frac{\gamma}{\pi(\omega^2+\gamma^2)}. \tag{S69}$$

Most of the terms in this sum do not survive projection into the zero-mode subspace. Recall that the solution of Eq. (S24) implies that

$$\boldsymbol{U}_\mu^\dagger \boldsymbol{\sigma}_3 \boldsymbol{\mathcal{V}}_{\mathbf{0},\alpha} \boldsymbol{\mathcal{V}}_{\mathbf{0},\alpha}^\dagger \boldsymbol{\sigma}_3 \boldsymbol{U}_\nu, \boldsymbol{U}_\mu^\dagger \boldsymbol{\sigma}_3 \boldsymbol{\mathcal{W}}_{\mathbf{0},\alpha} \boldsymbol{\mathcal{W}}_{\mathbf{0},\alpha}^\dagger \boldsymbol{\sigma}_3 \boldsymbol{U}_\nu \sim O(S^{-2}), \tag{S70}$$

for eigenvectors that do not arise from the zero mode subspace that appears in linear spin-wave theory. Since the energies, $E_{\mathbf{0},\alpha}$, outside the zero-mode subspace have a piece $\sim O(S)$, this means their total contribution to the first moment is $O(S^{-1})$ and thus can be ignored.

We thus can restrict only to those eigenvectors that arise from the zero mode subspace, which we denote as $\boldsymbol{\mathcal{V}}_0$ and $\boldsymbol{\mathcal{W}}_0$. We thus can write

$$\boldsymbol{U}_\mu^\dagger \boldsymbol{\sigma}_3 \left[ \int d\omega\, \omega\, \boldsymbol{A}(\mathbf{0},\omega) \right] \boldsymbol{\sigma}_3 \boldsymbol{U}_\nu = \boldsymbol{U}_\mu^\dagger \boldsymbol{\sigma}_3 \left[ \Delta \left( \boldsymbol{\mathcal{V}}_0 \boldsymbol{\mathcal{V}}_0^\dagger + \boldsymbol{\mathcal{W}}_0 \boldsymbol{\mathcal{W}}_0^\dagger \right) \right] \boldsymbol{\sigma}_3 \boldsymbol{U}_\nu + O(S^{-1}),$$

where $\Delta$ is the pseudo-Goldstone gap induced by spin-wave interactions. Note that we have set the width to zero for these modes; this is exact perturbatively in the interactions for the lowest lying mode, embodied in the assumption $\boldsymbol{\Sigma}^R(\mathbf{0},0) \sim \boldsymbol{\Sigma}^A(\mathbf{0},0)$ articulated in Sec. S2 A.

Since they are obtained via degenerate perturbation theory, the vectors $\boldsymbol{\mathcal{V}}_0$ and $\boldsymbol{\mathcal{W}}_0$ are related to the unperturbed eigenvectors, $\boldsymbol{V}_0$ and $\boldsymbol{W}_0$, by a change of basis. Because of this, one can show that the matrix elements that appear in the first moment are identical to those found upon projecting the sum of the effective dispersion matrix, $\boldsymbol{M}_0 + \boldsymbol{\Sigma}_0$ (see Sec. S2 A). Explicitly one finds

$$\boldsymbol{V}_0^\dagger [S\boldsymbol{M}_0 + \boldsymbol{\Sigma}_0] \boldsymbol{V}_0 = \boldsymbol{W}_0^\dagger [S\boldsymbol{M}_0 + \boldsymbol{\Sigma}_0] \boldsymbol{W}_0 = \boldsymbol{V}_0^\dagger \boldsymbol{\sigma}_3 \left( \Delta [\boldsymbol{\mathcal{V}}_0 \boldsymbol{\mathcal{V}}_0^\dagger + \boldsymbol{\mathcal{W}}_0 \boldsymbol{\mathcal{W}}_0^\dagger] \right) \boldsymbol{\sigma}_3 \boldsymbol{V}_0, \tag{S71a}$$

$$\boldsymbol{W}_0^\dagger [S\boldsymbol{M}_0 + \boldsymbol{\Sigma}_0] \boldsymbol{V}_0 = \left( \boldsymbol{V}_0^\dagger [S\boldsymbol{M}_0 + \boldsymbol{\Sigma}_0] \boldsymbol{W}_0 \right)^* = \boldsymbol{W}_0^\dagger \boldsymbol{\sigma}_3 \left( \Delta [\boldsymbol{\mathcal{V}}_0 \boldsymbol{\mathcal{V}}_0^\dagger + \boldsymbol{\mathcal{W}}_0 \boldsymbol{\mathcal{W}}_0^\dagger] \right) \boldsymbol{\sigma}_3 \boldsymbol{V}_0. \tag{S71b}$$

Using the sum rule [Eq. (S58)], and the definitions of $\boldsymbol{U}_\mu$ [Eq. (S55)] we can then see that

$$\boldsymbol{V}_0^\dagger [S\boldsymbol{M}_0 + \boldsymbol{\Sigma}_0] \boldsymbol{V}_0 = \frac{1}{2} \left[ \left( \frac{\partial^2 \epsilon_{\rm qu}}{\partial \theta^2} \right)_0 + \left( \frac{\partial^2 \epsilon_{\rm qu}}{\partial \phi^2} \right)_0 \right], \tag{S72a}$$

$$\boldsymbol{W}_0^\dagger [S\boldsymbol{M}_0 + \boldsymbol{\Sigma}_0] \boldsymbol{V}_0 = \frac{1}{2} \left[ \left( \frac{\partial^2 \epsilon_{\rm qu}}{\partial \theta^2} \right)_0 - \left( \frac{\partial^2 \epsilon_{\rm qu}}{\partial \phi^2} \right)_0 \right] - i \left( \frac{\partial^2 \epsilon_{\rm qu}}{\partial \theta \partial \phi} \right)_0. \tag{S72b}$$

The pseudo-Goldstone gap for the type II case is then found using Eq. (S28), giving the final result

$$\Delta = \sqrt{ \left( \frac{\partial^2 \epsilon_{\rm qu}}{\partial \theta^2} \right)_0 \left( \frac{\partial^2 \epsilon_{\rm qu}}{\partial \phi^2} \right)_0 - \left( \frac{\partial^2 \epsilon_{\rm qu}}{\partial \theta \partial \phi} \right)_0^2 } \sim O(S^0). \tag{S73}$$

### E. Type I pseudo-Goldstone mode

Finally, we consider the type I case. This is somewhat more involved given there is only a single soft-direction. We assume that the coordinates $\phi$ and $\theta$ are chosen such that $\theta = 0$, $\phi \neq 0$ represents the soft direction. Because of this, the spin-wave expansion is stable only for $\theta = 0$ and thus we have to be somewhat careful. Consider first the dependence on $\theta$ with $\phi = 0$

$$\mathcal{H}(0,\theta) = S^2 N \left[ \epsilon_{\rm cl}(0,0) + \frac{1}{2}\theta^2 \left( \frac{\partial^2 \epsilon_{\rm cl}}{\partial \theta^2} \right)_0 \right] + O(S). \tag{S74}$$

We thus see that there is an $O(S^2)$ contribution to this second derivative, with

$$\frac{1}{SN}\left\langle\left(\frac{\partial^2\mathcal{H}}{\partial\theta^2}\right)_0\right\rangle = S\left(\frac{\partial^2\epsilon_{\rm cl}}{\partial\theta^2}\right)_0 + O(S^0). \tag{S75}$$

Next consider the case where $\theta = 0$, but $\phi \neq 0$, where there is no classical contribution, but a well defined spin-wave expansion at $O(S)$. One writes

$$\mathcal{H}(\phi, 0) = S(S+1)N\epsilon_{\rm cl}(0,0) + SN\epsilon_{\rm qu}(\phi,0) + S\sum_{\boldsymbol{k}\alpha}\epsilon_{\boldsymbol{k}\alpha}(\phi,0)\gamma^\dagger_{\boldsymbol{k}\alpha}\gamma_{\boldsymbol{k}\alpha} + O(S^{1/2}). \tag{S76}$$

Following the discussion in Sec. S7, we can then see that

$$\frac{1}{SN}\left\langle\left(\frac{\partial^2\mathcal{H}}{\partial\phi^2}\right)_0\right\rangle = \left(\frac{\partial^2\epsilon_{\rm qu}}{\partial\phi^2}\right)_0 + O(S^{-1}). \tag{S77}$$

Now all that remains is the cross-term. The classical part of this vanishes due to the choice of $\phi$ is the soft mode direction. Going beyond the classical part requires the handling of terms linear in the magnons, as in Sec. S3 A. In this case the only piece of interest is the $O(S^{3/2})$ part, however, this is at most of order $O(\theta\phi)$, and since $\langle a_{\boldsymbol{0},\alpha}\rangle = O(S^{-1/2})$, this contribution is at most $O(S)$, with

$$\frac{1}{SN}\left\langle\left(\frac{\partial^2\mathcal{H}}{\partial\theta\partial\phi}\right)_0\right\rangle = O(S^0). \tag{S78}$$

Due to the presence of the classical, $O(S^2)$, parts of the curvatures, this has no effect at leading order and thus can be ignored. Following the results of Sec. S3 D, we then can write

$$\boldsymbol{V}_0^\dagger[S\boldsymbol{M}_0 + \boldsymbol{\Sigma}_0]\boldsymbol{V}_0 = \frac{1}{2}\left[S\left(\frac{\partial^2\epsilon_{\rm cl}}{\partial\theta^2}\right)_0 + \left(\frac{\partial^2\epsilon_{\rm qu}}{\partial\phi^2}\right)_0\right], \tag{S79a}$$

$$\boldsymbol{W}_0^\dagger[S\boldsymbol{M}_0 + \boldsymbol{\Sigma}_0]\boldsymbol{V}_0 = \frac{1}{2}\left[S\left(\frac{\partial^2\epsilon_{\rm cl}}{\partial\theta^2}\right)_0 - \left(\frac{\partial^2\epsilon_{\rm qu}}{\partial\phi^2}\right)_0\right]. \tag{S79b}$$

We thus have the final result, following Eq. (S31),that

$$\Delta = S^{1/2}\sqrt{\left(\frac{\partial^2\epsilon_{\rm cl}}{\partial\theta^2}\right)_0\left(\frac{\partial^2\epsilon_{\rm qu}}{\partial\phi^2}\right)_0} + O(S^{-1/2}). \tag{S80}$$

## S4. REMARKS ON SOME CONNECTIONS TO QUANTUM CHROMODYNAMICS

The curvature formula presented in this paper bears some similarity to various formulas appearing in the literature on quantum chromodynamics (QCD) and chiral perturbation theory. Since, as it turns out, the similarities are more than merely superficial we briefly remark on them here.

Our work rests on the existence of accidental degeneracies in frustrated magnets which are not protected by symmetries of the full Hamiltonian. An analogous situation arises in the physics of the strong nuclear force [5]: when the bare $u$, $d$, $s$ quark masses are set to zero there is a set of global symmetries associated with axial charges – one for each of the eight generators of

SU(3) – with 3 being the number of quark flavors. Although not exact symmetries of nature, it is fruitful to think along these lines because, in doing so, one realizes that the global symmetries are spontaneously broken leading to eight Goldstone modes. These can be associated with the lightest meson octet consisting of the $\pi$, $K$ and $\eta$ mesons – their masses arising from the explicit breaking of the axial vector symmetries. A formula due to Dashen [6]

$$m^2 \propto \langle [Q_5 \, [Q_5, \mathcal{H}]] \rangle \,, \tag{S81}$$

relates the meson mass to a double commutator of the Hamiltonian with generators of the approximate symmetries. The more widely known Gellmann-Oakes-Renner formula [7] follows from this relation. Dashen's formula is analogous to the left-hand side of sum rule formula [Eq. (S58)], relating the first-moment of the spectral function to the gap of pseudo-Goldstone mode. In the context of QCD, the part of the Hamiltonian $\mathcal{H}$ that contributes to the mass comes from the explicit symmetry-breaking terms, such as the quark masses.

In addition to the physics of spontaneous and explicit breaking of SU(3) axial vector currents, there is a classically conserved U(1) axial charge which is broken by quantum fluctuations. Accordingly, there is also a ninth pseudoscalar meson $\eta'$ with a mass significantly larger than that of the pseudoscalar octet. Witten and Veneziano [8, 9] addressed the question of how to precisely frame the $\eta'$ mass as arising from the anomaly. Schematically, in the large-$N$ limit of SU($N$) Yang-Mills theory with massless quarks one finds [8]

$$m_{\eta'}^2 \propto \left[ \frac{\partial^2 \epsilon_{\rm YM}}{\partial \theta^2} \right]_0 \equiv \chi_\infty \propto \frac{1}{N}, \tag{S82}$$

where $m_{\eta'}$ is the mass of the $\eta'$-meson and $\chi_\infty$ is the "topological susceptibility": the curvature of the energy of the pure gauge system with respect to the addition of the topological $\theta$-term that is associated with the U(1) anomaly [8]. In broad strokes this resembles the curvature formula: specifically, the $\eta'$ mass is analogous to the pseudo-Goldstone gap, and $\chi_\infty$ is analogous to the (mean) curvature of the classical and quantum zero-point energy densities and $N$ is analogous to $S$. The proof we give here for the pseudo-Goldstone gap is in a similar spirit to the argument presented by Witten: as in our case where a mixing of orders in perturbation theory ensures that the ground state energy is independent of the spin configuration, the small meson mass $m_{\eta'}^2 \sim 1/N$, is needed to cancel a term at $O(N^2)$ to render the total energy independent of the $\theta$ angle [8].

We note in passing that order-by-disorder as discussed in condensed matter is similar to the notion of an anomaly in field theory in the sense that both involve the lifting of a classical symmetry by fluctuations. The resemblance is no deeper than this however, as while anomalies stem from the lack of invariance of the path integral measure, in the case of order-by-disorder accidental symmetries can usually be fine-tuned to become exact symmetries. Even so, the story of understanding the $\eta'$ mass in large-$N$ QCD from the axial U(1) anomaly does have some interesting parallels to our work.

## S5. ORDER-BY-QUANTUM DISORDER MODELS

We now discuss some details of the explicit calculations of the pseudo-Goldstone gap in a number of relevant quantum spin models. Where possible we will compare with other theoretical approaches or directly with experimental data. The key results have been presented in Table I of the main text.

### A. Heisenberg-compass models

The simplest, and one of the earliest studied cases [10, 11] of order-by-quantum-disorder is a Heisenberg ferromagnet with a compass type anisotropy on square or cubic lattices. We write these models as

$$\sum_{i\mu}\left[J\boldsymbol{S}_i\cdot\boldsymbol{S}_{i+\mu}+KS^{\mu}_{i}S^{\mu}_{i+\mu}\right], \tag{S83}$$

where $J<0$ is ferromagnetic and $\mu$ is the bond direction. For $K=0$ the classical ground state is a ferromagnet, $\boldsymbol{S}_i = S\hat{\boldsymbol{n}}$, with arbitrary overall direction $\hat{\boldsymbol{n}}$. In the square lattice case, finite $K>0$ selects $\hat{\boldsymbol{n}}=\hat{\boldsymbol{z}}$, with no residual degeneracy, while $K<0$ fixes $\hat{\boldsymbol{n}}$ to the $\hat{\boldsymbol{x}}$-$\hat{\boldsymbol{y}}$ plane with a U(1) degeneracy. This is lifted by the quantum zero-point energy to select states aligned with the cubic axes, $\hat{\boldsymbol{n}}=\hat{\boldsymbol{x}},\hat{\boldsymbol{y}}$, with the associated pseudo-Goldstone mode being type I. A similar picture holds in the cubic case, except there is a residual type II $O(3)$ degeneracy for either sign of $K$, with the zero-point energy selecting the cubic axes [11]. As shown in Table I of the main text, the induced pseudo-Goldstone gap appears at next order in $1/S$. For small $|K|/|J|$ this yields a gap $\Delta \propto S^{1/2}|K|^{3/2}/|J|^{1/2}$ for the square lattice and $\Delta\propto K^2/|J|$ for the cubic lattice. Note that for both square and cubic models, the three-magnon interactions vanish, and thus there is no magnon decay.

We should note that the cubic-compass model was studied by Belorizky *et al.* [11], where order-by-quantum-disorder selection was computed, as well as the gap of the pseudo-Goldstone modes due to spin-wave interactions. In fact, a similar problem, order-by-quantum-disorder in cubic dipolar ferromagnets, was studied by Tessman [10], predating by several decades the seminal works of Villain *et al.* [12], Henley [13] and Shender [14]. The results of Belorizky *et al.* [11] are in quantitative agreement with ours where they overlap (see Table I of the main text and Eq. (29) of Ref. [11]). In their work, the relationship between the zero-point curvature and the gap was noted, and an argument was given for why this occurred. Their argument has some implicit assumptions that make it (a) incomplete and (b) not generalizable to the arbitrary order-by-quantum-disorder scenarios.

### B. Heisenberg-Kitaev-Γ models

Another Heisenberg-compass model that has attracted recent attention is the Heisenberg-Kitaev [15] model and the related Heisenberg-Kitaev-Γ model [16] defined on the honeycomb

lattice. This reads

$$\sum_{\langle ij\rangle\in\alpha\beta(\gamma)} \left[ J\boldsymbol{S}_i\cdot\boldsymbol{S}_j + KS_i^{\gamma}S_j^{\gamma} + \Gamma\left(S_i^{\alpha}S_j^{\beta} + S_i^{\beta}S_j^{\alpha}\right)\right], \tag{S84}$$

where the bonds have been divided into three types: $(x)yz$, $x(y)z$ and $xy(z)$, as defined in Ref. [16].

First consider the Heisenberg-Kitaev limit, where $\Gamma = 0$. As a function of $J$ and $K$ there are four classical phases, a ferromagnet, anti-ferromagnet and the so-called zigzag and stripy phases [17]. All of these states have an accidental classical $O(3)$ degeneracy that is lifted by quantum fluctuations. In all cases the selection pins the moment direction to lie along the cubic spin axes [15, 17]. Since the stripy and zigzag phases can be mapped to the ferromagnet and antiferromagnet via a duality, and therefore do not need to be studied separately. The ferromagnetic case is similar to the cubic compass ferromagnet, showing a type II pseudo-Goldstone gap that scales as $\Delta \propto K^2/J$. The anti-ferromagnetic case is subtler: the Heisenberg limit has *two* type I Goldstone modes that are lifted by the introduction of the Kitaev exchange $K$. These two modes are lifted identically and do not mix, with their gap scaling strongly with the Kitaev exchange, going as $\Delta \propto |K|S^{1/2}$. Both these cases do not have three-magnon interactions due to a residual $C_2$ spin rotation symmetry.

The phase diagram is more complex when $\Gamma \neq 0$, with many of the accidental degeneracies of the Heisenberg-Kitaev limit lifted [16]. We consider a region near the ferromagnetic limit where $J < 0$, $K = 0$ and $\Gamma > 0$. Here the spins are uniform, $\boldsymbol{S}_i = S\hat{\boldsymbol{n}}$, in the plane perpendicular to [111] with arbitrary orientation [16]. This accidental degeneracy is lifted by the quantum zero-point energy selecting directions equivalent to $\hat{\boldsymbol{n}} = (\boldsymbol{y}-\boldsymbol{x})/\sqrt{2}$. The pseudo-Goldstone mode is type I, with a gap that scales as $\Delta \sim S^{1/2}\Gamma^2/|J|$. We note that, in contrast to the other cases discussed so far, this model includes three-magnon interaction terms and thus magnon decay.

### C. $J_1$-$J_2$ models

Next, we consider one of the paradigmatic models of quantum-order-by-disorder, the $J_1$-$J_2$ anti-ferromagnet on the square lattice [13, 18]

$$J_1\sum_{\langle ij\rangle}\boldsymbol{S}_i\cdot\boldsymbol{S}_j + J_2\sum_{\langle\langle ij\rangle\rangle}\boldsymbol{S}_i\cdot\boldsymbol{S}_j. \tag{S85}$$

While the behavior of this model has been extensively studied for $S = 1/2$ (for example, see Refs. [19–34]), we focus here on large-$S$ limit where a semi-classical analysis applies. For $J_1/J_2 = 0$ one sees that the two sublattices of the square lattices decouple and form two independent Néel anti-ferromagnets, with the relative orientation unconstrained. At the classical level this remains true for large $J_2$, until the transition to the usual Néel state at $J_1 = 2J_2$. There is thus an $O(3)$ degeneracy which, at leading order in $1/S$ is lifted by quantum fluctuations, in addition to the overall $O(3)$ due to spin rotation invariance. As shown by Henley [13], these fluctuations select a colinear state, with the two sublattices either aligned or anti-aligned. We note that in the spin-1/2 case, while the Néel and colinear stripe phases appear for small and large $J_2/J_1$ (respectively), they are separated by a non-magnetic intermediate phase, occupying the range $0.4 \lesssim J_2/J_1 \lesssim 0.6$ [31].

Like the Heisenberg-Kitaev case, this has a pair of type-I pseudo-Goldstone modes, but, in addition, a pair of type I true Goldstone modes that remain gapless. As shown in Table I of the main text, the gap scales as $\Delta \propto J_1 S^{1/2}$ for $J_1 \ll J_2$, matching the appropriately defined mean curvature exactly. This case has also been studied in the $S = 1/2$ limit by series expansion techniques [35]. One finds that the relevant gap to triplet excitations (with $S = 1/2$) is in reasonable agreement with our $O(1/S^2)$ spin-wave results (see Table I of the main text).

The $J_1$-$J_2$ model on the triangular lattice has similar physics, though the classical ground state manifold is a bit more complex [36]. As in the case of the square lattice, there have been extensive studies of the $S = 1/2$ limit of this model [37–47] which we will not broach in detail here. Classically, for small $J_2/J_1$ one finds the usual 120° structure, while for large $J_2/J_1$ one finds an incommensurate state [48]. At intermediate values, in the range $1/8 < J_2/J_1 < 1$ the classical ground state consists of any state in which the sum of the four spins on each rhombus of the lattice is zero [48]. This degeneracy is lifted by order-by-disorder, picking the maximally colinear state consisting of alternating ferromagnetic stripes [13, 36]. This has a pair of type II pseudo-Goldstone modes, in addition to a pair of type I true Goldstone modes that remain gapless. As shown in Table I of the main text, the gap scales as $\Delta \propto J_1 S^0$, and is largest near the boundaries, with a minimum of $\Delta \sim 0.44 J_1$ near $J_2/J_1 \sim 0.42$. Similar to the square lattice case, we note that for spin-1/2 while the 120° Néel and colinear stripe phases appear at small and large $J_2/J_1$, an intermediate phase appears inbetween. This intermediate phase, thought to be quantum spin liquid, occupies the region $0.06 \lesssim J_2/J_1 \lesssim 0.17$ [43, 44].

### D. $Ca_3Fe_2Ge_3O_{12}$

We now consider an experimental candidate for order-by-quantum-disorder in a real materials, the garnet $Ca_3Fe_2Ge_3O_{12}$ [14, 49–52]. The magnetic ions in $Ca_3Fe_2Ge_3O_{12}$ are (spin-only) $Fe^{3+}$ ions ($S = 5/2$), which form a pair of interpenetrating simple cubic lattices. Each site has only a single three-fold axis, thus there are two types of nearest-neighbor exchanges ($J_1$ and $J_1'$) and one second-neighbor exchange ($J_2$) [49]. We write this model schematically as

$$J_1 \sum_{\langle ij \rangle_{\parallel}} \boldsymbol{S}_i \cdot \boldsymbol{S}_j + J_1' \sum_{\langle ij \rangle_{\perp}} \boldsymbol{S}_i \cdot \boldsymbol{S}_j + J_2 \sum_{\langle\langle ij \rangle\rangle} \boldsymbol{S}_i \cdot \boldsymbol{S}_j, \tag{S86}$$

where the first neighbors $\langle ij \rangle$ have been partitioned into those along the local three-fold axis, denoted as $\langle ij \rangle_{\parallel}$, and those perpendicular to it, denoted as $\langle ij \rangle_{\perp}$. These parameters have been estimated by comparison with the inelastic neutron scattering spectrum at zero field, where it was found that [49]

$$J_1 = 0.156 \text{ meV}, \qquad J_1' = 0.053 \text{ meV}, \qquad J_2 = 0.106 \text{ meV},$$

reproduces the experimental spectrum reasonably well. Note that these numbers have been doubled relative to those presented in Ref. [49], to account for a double counting of the bonds. The

classical ground states consist of two independent Néel antiferromagnets on the two cubic sublattices.

The order-by-disorder physics in this material is a three-dimensional analogue of the $J_1$-$J_2$ square lattice model and has the same basic features: selection of colinear ordering and gapping of two type I pseudo-Goldstone modes. For the experimental parameters we find the gap is given by

$$\Delta = 166\,\mu\text{eV} \cdot S^{1/2} + O(S^{-1/2}), \tag{S87}$$

giving $\sim 262\,\mu$eV for $S = 5/2$. This is in rough agreement with the gap of 0.033THz = 136 $\mu$eV that has been observed experimentally [49]. There are some alternatives to an interpretation in terms of order-by-quantum-disorder – biquadratic exchange can directly lift the accidental degeneracy [53]. The fact that the predicted gap is *larger* than found in experiment, coupled with the relatively large spin $S = 5/2$, suggests such classical selection effects may not necessary, but perhaps the fitted parameters or the exchanges included in the model may need to be revisited. One concern is that the fit used to obtain the exchange parameters was performed using linear spin-wave theory at zero-field [51], neglecting the effect of interactions, rather than in a limit where these effects are controlled (e.g. high magnetic field). Another concern is that the temperature at which the experiments were done is moderate relative to the induced gap size [49, 51], raising questions to whether thermal effects also have to be considered. Additional terms in the model itself may also be necessary, e.g. a (positive) biquadratic exchange or perhaps some type of anisotropic exchange could also have the effect of lowering the predicted gap size. Finally, there is also the possibility that, despite the spin being rather large ($S = 5/2$), the computation of the pseudo-Goldstone gap at leading order in $1/S$ may not be quantitative.

We note that the classical part of the curvatures can be worked out analytically, with $\left(\frac{\partial^2 \epsilon}{\partial \theta^2}\right)_0 = S^2(12J_2 - 2(J_1 + 3J_1'))$, while $\left(\frac{\partial^2 \epsilon}{\partial \phi^2}\right)_0$ must be computed numerically. As in the examples discussed earlier, to do this we compute the zero-point energy $\epsilon(0, \phi)$ for a number of small but finite values of $\phi$ and fit to a polynomial to extract the curvature. This model includes only four-magnon interactions, with the three-magnon terms vanishing due to the isotropic interactions and colinear ground state.

### E. $Er_2Ti_2O_7$

Finally, we consider the XY anti-ferromagnet $Er_2Ti_2O_7$ which is a leading candidate for experimental realization of order-by-quantum disorder. The appropriate pseudo-spin-1/2 model for the $Er^{3+}$ ions take the form

$$\sum_{\langle ij\rangle} [J_{zz} S_i^z S_j^z - J_{\pm}\left(S_i^+ S_j^- + S_i^- S_j^+\right) + \\ J_{\pm\pm}\left(\gamma_{ij} S_i^+ S_j^+ + \text{h.c.}\right) + J_{z\pm}\left(\zeta_{ij}\left[S_i^z S_j^+ + S_i^+ S_j^z\right] + \text{h.c.}\right)].$$

The exchange parameters have been determined by fitting the spin-wave spectrum in an applied magnetic field. Good agreement is found for the values [53]

$$J_{zz} = -2.5 \cdot 10^{-2}\ \text{meV}, \qquad J_{\pm} = +6.5 \cdot 10^{-2}\ \text{meV},$$
$$J_{\pm\pm} = +4.2 \cdot 10^{-2}\ \text{meV}, \qquad J_{z\pm} = -0.88 \cdot 10^{-2}\ \text{meV}, \tag{S88}$$

where the phases $\gamma_{ij}$, $\zeta_{ij}$ and lattice structure are given in detail in Ref. [53]. The classical ground states have the pseudo-spins uniformly in their local XY planes, $\boldsymbol{S}_i = S\,(\cos\phi\hat{\boldsymbol{x}} + \sin\phi\hat{\boldsymbol{y}})$, with the overall angle, $\phi$, arbitrary. Order-by-quantum-disorder selects the six so-called $\psi_2$ states, with $\phi = n\pi/3$ ($n = 0, 1, \ldots, 5$) and yields a single type I pseudo-Goldstone mode, similar in spirit to the square compass ferromagnet discussed earlier. This has been argued to be one of the best cases for observing order-by-quantum-disorder as two-spin interactions of arbitrary range do not lift the classical degeneracy. For these exchange parameters one finds the gap to be

$$\Delta = 44\,\mu\text{eV} \cdot S^{1/2} + O(S^{-1/2}) \tag{S89}$$

giving $\sim 31\ \mu$eV for $S = 1/2$. This number is comparable, though somewhat smaller, than the gaps that have been reported from experiment, which range from 43 $\mu$eV [54] to 53 $\mu$eV [55]. We note that the classical curvature $\left(\frac{\partial^2\epsilon}{\partial\theta^2}\right)_0$ can be computed analytically, giving $\left(\frac{\partial^2\epsilon}{\partial\theta^2}\right)_0 = 6(2J_{\pm} + J_{zz})S^2$, while $\left(\frac{\partial^2\epsilon}{\partial\phi^2}\right)_0$ must be computed numerically. As discussed previously, to do this we compute the zero-point energy $\epsilon(0, \phi)$ for a number of small but finite values of $\phi$ and fit to a polynomial to extract the curvature. We note that this case includes both three- and four-magnon interactions due to the highly anisotropic exchange interactions.

## S6. CURVATURE CALCULATION EXAMPLES

In this Section we give a selection of representative cases on how to calculate the curvatures for the examples discuss in in the Table I of the main text. For the sake of brevity we adopt the shorthand for the curvatures

$$\left(\frac{\partial^2\epsilon}{\partial\theta^2}\right)_0 \equiv A_{\theta\theta}, \qquad \left(\frac{\partial^2\epsilon}{\partial\phi^2}\right)_0 \equiv A_{\phi\phi}, \qquad \left(\frac{\partial^2\epsilon}{\partial\theta\partial\phi}\right)_0 \equiv A_{\theta\phi}, \tag{S90}$$

as well as for the transverse part of the soft-mode configuration

$$\boldsymbol{S}_\alpha = S\left(\phi\hat{\boldsymbol{x}}_\alpha + \theta\hat{\boldsymbol{y}}_\alpha + \hat{\boldsymbol{z}}_\alpha\left[1 - (\phi^2 + \theta^2)\right]^{1/2}\right) \equiv \boldsymbol{S}^\perp_\alpha + S\,\hat{\boldsymbol{z}}_\alpha\left(1 - \frac{|\boldsymbol{S}^\perp_\alpha|^2}{S^2}\right)^{1/2}. \tag{S91}$$

### A. Heisenberg-compass (cubic, ferromagnet)

This example is particularly simple, since there is a single sublattice and it is type II. Expanding about a state with ordering vector along the cubic $\hat{\boldsymbol{z}}$ axis it is clear that the relevant states are

$$\boldsymbol{S}^\perp_i = S\left[\phi\hat{\boldsymbol{x}} + \theta\hat{\boldsymbol{y}}\right]. \tag{S92}$$

We see then the curvatures correspond to simply rotating the ordering direction along the $\hat{\boldsymbol{x}}$ and $\hat{\boldsymbol{y}}$ directions. Due to the cubic symmetry this then further implies that $A_{\theta\theta} = A_{\phi\phi} \equiv A$, with $A_{\theta\phi} = 0$, giving a gap equation $\Delta = A/S$. To compute $A$ we compute $\epsilon_{\rm qu}(\theta, 0)$ numerically for a series of small values of $\theta$, fitting to a quadratic form to extract the curvature.

### B. $J$-$\Gamma$ model (honeycomb, ferromagnet)

This is a particular limit ($K = 0$) of the $J$-$K$-$\Gamma$ model [16] discussed in Sec. S5 B. For $J < 0$ and $\Gamma > 0$ it orders ferromagnetically into the plane perpendicular to [111] and thus has a superficially more complicated structure. We define the vectors

$$\boldsymbol{X} = \frac{1}{\sqrt{6}}\left[\hat{\boldsymbol{x}} + \hat{\boldsymbol{y}} - 2\hat{\boldsymbol{z}}\right], \tag{S93a}$$

$$\boldsymbol{Y} = \frac{1}{\sqrt{2}}\left[\hat{\boldsymbol{y}} - \hat{\boldsymbol{x}}\right], \tag{S93b}$$

$$\boldsymbol{Z} = \frac{1}{\sqrt{3}}\left[\hat{\boldsymbol{x}} + \hat{\boldsymbol{y}} + \hat{\boldsymbol{z}}\right]. \tag{S93c}$$

The selected ferromagnetic ground state for $\Gamma > 0$ is along $\hat{\boldsymbol{Y}}$ (and its equivalents) so we parameterize

$$\hat{\boldsymbol{x}}_A = -\hat{\boldsymbol{X}}, \qquad \hat{\boldsymbol{y}}_A = \hat{\boldsymbol{Z}}, \qquad \hat{\boldsymbol{z}}_A = \hat{\boldsymbol{Y}}, \tag{S94a}$$

$$\hat{\boldsymbol{x}}_B = -\hat{\boldsymbol{X}}, \qquad \hat{\boldsymbol{y}}_B = \hat{\boldsymbol{Z}}, \qquad \hat{\boldsymbol{z}}_B = \hat{\boldsymbol{Y}}. \tag{S94b}$$

The relevant spin configurations are thus given by

$$\boldsymbol{S}^{\perp}_{i,A} = \boldsymbol{S}^{\perp}_{i,B} = S\left[-\phi\hat{\boldsymbol{X}} + \theta\hat{\boldsymbol{Z}}\right]. \tag{S95}$$

The classical contributions to the curvatures are thus simply given by

$$A_{\theta\theta} = 3\Gamma S^2, \tag{S96}$$

with $A_{\phi\phi} \sim O(S)$ generated only by quantum fluctuations, as given in Table I of the main text. To compute $A_{\phi\phi}$ we computed $\epsilon_{\rm qu}(\phi, 0)$ numerically for the spin configurations above for a series of small values of $\phi$. We then fit these values to a quadratic form to extract the curvature.

### C. Heisenberg $J_1$-$J_2$ (square, stripe)

This example has two true type I Goldstone modes in addition to two type I pseudo-Goldstone modes. These modes are described by a unit cell with four sites, which we label as $A$ (at $\boldsymbol{0}$), $B$ (at $\hat{\boldsymbol{x}}$), $C$ (at $\hat{\boldsymbol{y}}$) and $D$ (at $\hat{\boldsymbol{x}} + \hat{\boldsymbol{y}}$). The stripe, $(\pi, 0)$ order is then given by the vectors

$$\hat{\boldsymbol{z}}_A = \hat{\boldsymbol{z}}_D = +\hat{\boldsymbol{z}}, \qquad \hat{\boldsymbol{z}}_B = \hat{\boldsymbol{z}}_C = -\hat{\boldsymbol{z}}. \tag{S97}$$

The pseudo-Goldstone modes of interest are those that change the relative angle of the two sublattices. The appropriate local frames for one of these modes is then given by

$$\hat{\boldsymbol{x}}_A = \hat{\boldsymbol{x}}_B = +\hat{\boldsymbol{x}}, \qquad \hat{\boldsymbol{x}}_C = \hat{\boldsymbol{x}}_D = -\hat{\boldsymbol{x}},$$
$$\hat{\boldsymbol{y}}_A = \hat{\boldsymbol{y}}_D = +\hat{\boldsymbol{y}}, \qquad \hat{\boldsymbol{y}}_B = \hat{\boldsymbol{y}}_C = -\hat{\boldsymbol{y}}, \tag{S98}$$

as in the Néel case, the second soft mode is identical in character, with the role of $\hat{\boldsymbol{x}}$ and $\hat{\boldsymbol{y}}$ axes switched. These define the soft spin configurations

$$\boldsymbol{S}^{\perp}_{i,A} = S\left[+\phi\hat{\boldsymbol{x}} + \theta\hat{\boldsymbol{y}}\right], \qquad \boldsymbol{S}^{\perp}_{i,B} = S\left[+\phi\hat{\boldsymbol{x}} - \theta\hat{\boldsymbol{y}}\right],$$
$$\boldsymbol{S}^{\perp}_{i,C} = S\left[-\phi\hat{\boldsymbol{x}} - \theta\hat{\boldsymbol{y}}\right], \qquad \boldsymbol{S}^{\perp}_{i,D} = S\left[-\phi\hat{\boldsymbol{x}} + \theta\hat{\boldsymbol{y}}\right]. \tag{S99}$$

This then yields the classical curvature for the $\theta$ direction as

$$A_{\theta\theta} = 4(2J_2 - J_1)S^2, \tag{S100}$$

with the classical curvature $A_{\phi\phi} \sim O(S)$, as given in Table I of the main text. To compute $A_{\phi\phi}$ we computed $\epsilon_{\text{qu}}(\phi, 0)$ numerically for the spin configurations above for a series of small values of $\phi$. We then fit these values to a quadratic form to extract the curvature.

## S7. WORKED EXAMPLE: HEISENBERG-COMPASS MODEL ON SQUARE LATTICE

To illustrate the formalism in full detail, we present a complete worked example for the case of the Heisenberg-compass model on the square lattice, as discussed in Sec. S5 A. We consider the model

$$H = \sum_i \sum_{\mu=x,y} \left[J\boldsymbol{S}_i \cdot \boldsymbol{S}_{i+\mu} + KS^{\mu}_i S^{\mu}_{i+\mu}\right], \tag{S101}$$

where $J < 0$ and $K < 0$. The classical ground states ($1/S \to 0$) consist of the spins being uniform in the $\hat{\boldsymbol{x}}$-$\hat{\boldsymbol{y}}$ plane

$$\boldsymbol{S}_i \equiv S\left(\cos\phi\hat{\boldsymbol{x}} + \sin\phi\hat{\boldsymbol{y}}\right). \tag{S102}$$

Consider spin-wave theory about such a state. We define the local frames, as in Sec. S1, to be

$$\hat{\boldsymbol{x}}_i \equiv -\sin\phi\hat{\boldsymbol{x}} + \cos\phi\hat{\boldsymbol{y}}, \qquad \hat{\boldsymbol{y}}_i \equiv \hat{\boldsymbol{z}}, \qquad \hat{\boldsymbol{z}}_i \equiv \cos\phi\hat{\boldsymbol{x}} + \sin\phi\hat{\boldsymbol{y}}. \tag{S103}$$

The linear spin-wave Hamiltonian (leading order in $1/S$) can be written

$$H = S\sum_{ij}\left[A_{ij}a^{\dagger}_i a_j + \frac{1}{2}\left(B_{ij}a^{\dagger}_i a^{\dagger}_j + \text{h.c.}\right)\right] + \text{const.} \tag{S104}$$

then we have (see Sec. S1)

$$A_{i,i+x} = J + \frac{K}{4}\left(1 - \cos 2\phi\right), \qquad A_{i,i+y} = J + \frac{K}{4}\left(1 + \cos 2\phi\right), \tag{S105a}$$
$$B_{i,i+x} = \frac{K}{2}\sin^2\phi, \qquad B_{i,i+y} = \frac{K}{2}\cos^2\phi, \tag{S105b}$$
$$A_{ii} = 2J + K, \qquad B_{ii} = 0. \tag{S105c}$$

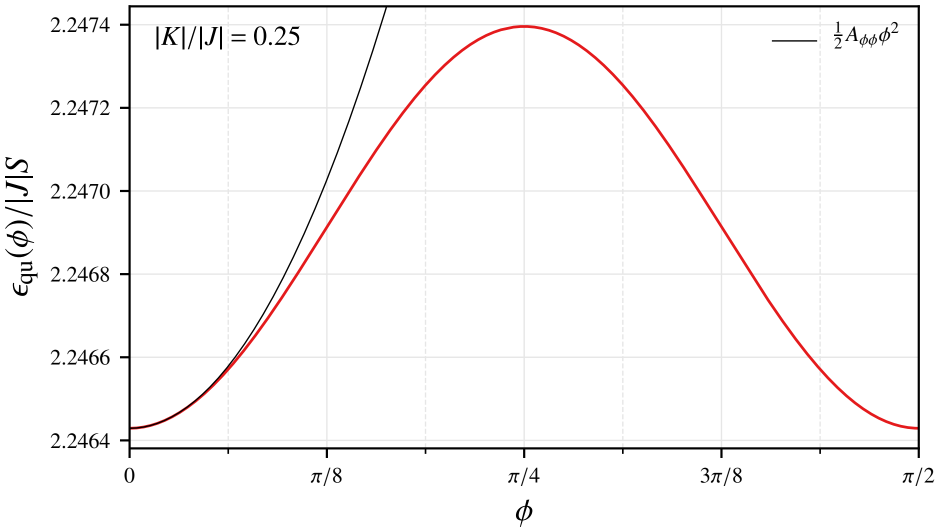


FIG. S1. Zero-point energy of the Heisenberg-compass model on the square lattice with $J < 0$ and $K < 0$ and $|K|/|J| = 0.25$. The angle $\phi$ parametrizes the classical ground state spin configuration, as given in Eq. (S102). The minima of the zero-point energy are given by the Cartesian axes $\pm\hat{\boldsymbol{x}}$, $\pm\hat{\boldsymbol{y}}$ corresponding to the angles $\phi = 0, \pi/2, \pi$ or $3\pi/2$. The curvature, $A_{\phi\phi} \approx 0.00775|J|S$, can be found numerically by fitting a polynomial near $\phi = 0$.

The appropriate Fourier transforms of these quantities are given by

$$A_{\boldsymbol{k}}(\phi) \equiv \left(2J + \frac{K}{2}\right)\left(\cos k_x + \cos k_y\right) + \frac{K}{2}\cos 2\phi\left(\cos k_y - \cos k_x\right) - 2(2J + K), \tag{S106a}$$

$$B_{\boldsymbol{k}}(\phi) \equiv K\left(\cos k_x \sin^2\phi + \cos k_y \cos^2\phi\right). \tag{S106b}$$

The spin-wave dispersion is then simply given by

$$\epsilon_{\boldsymbol{k}}(\phi) = \left(A_{\boldsymbol{k}}(\phi)^2 - B_{\boldsymbol{k}}(\phi)^2\right)^{1/2}. \tag{S107}$$

Note that since $A_{\boldsymbol{0}}(\phi) = -B_{\boldsymbol{0}}(\phi) = -K$ one has $\epsilon_{\boldsymbol{0}}(\phi) = 0$, indicating a (type I) pseudo-Goldstone mode.

By direct calculation one can see that the minimum of the zero-point energy occurs when $\phi = 0, \pi/2, \pi$ or $3\pi/2$, i.e. along the cubic axes (see Fig. S1). Focus on $\phi = 0$, where the conjugate direction is simply rotating the spins out of the $\hat{\boldsymbol{x}}$-$\hat{\boldsymbol{y}}$ plane. As in the examples presented in Sec. S6, one can compute that the classical curvature is $A_{\theta\theta} = 2|K|S^2$. Computing the curvature of the zero-point energy can be done in several ways. The most widely applicable is to simply compute $\epsilon_{\rm qu}(\phi)$ on a dense grid of $\phi$ and extract the curvature by fitting a polynomial in $\phi$. Such a fit is shown in Fig. S1. Note that more generally the diagonalization needed to obtain the spin-wave energies, $\epsilon_{\boldsymbol{k}}$, may also need to be carried out numerically.

However, since the the current problem is rather simple we can go a little further analytically. First one can note that $A_{\boldsymbol{k}}(0) = 2J\cos k_x + (2J + K)(\cos k_y - 2)$ and $B_{\boldsymbol{k}}(0) = 2K\cos k_y$. To evaluate

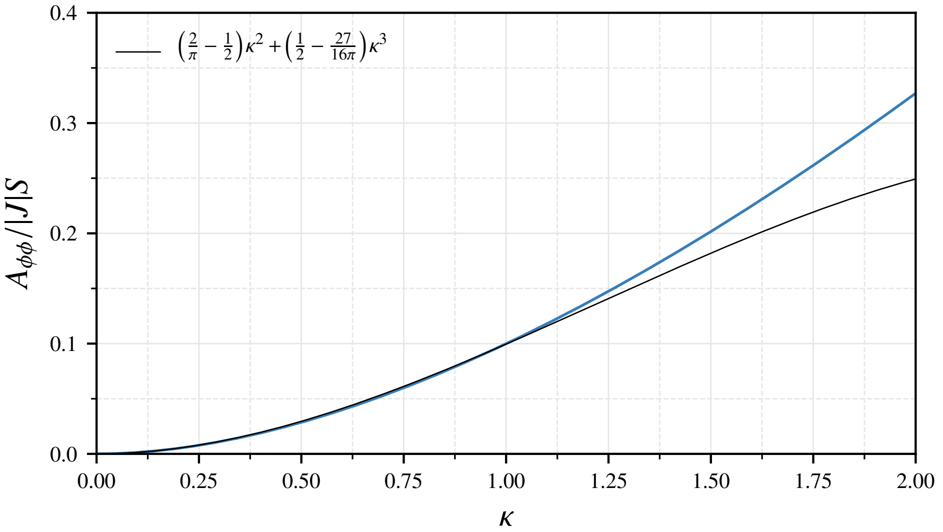


FIG. S2. The curvature of the zero-point energy ($A_{\phi\phi}$) of the Heisenberg-compass model on the square lattice with $J < 0$ and $K < 0$ as a function of $\kappa \equiv |K|/|J|$. The asymptotic form for $\kappa \ll 1$ is also shown.

the curvature of the zero-point energy we carry out the derivatives with respect to $\phi$ analytically. One finds

$$\left(\frac{\partial A_{\boldsymbol{k}}(\phi)}{\partial \phi}\right)_{\phi=0} = \left(\frac{\partial B_{\boldsymbol{k}}(\phi)}{\partial \phi}\right)_{\phi=0} = 0, \tag{S108}$$

$$\left(\frac{\partial^2 A_{\boldsymbol{k}}(\phi)}{\partial \phi^2}\right)_{\phi=0} = \left(\frac{\partial^2 B_{\boldsymbol{k}}(\phi)}{\partial \phi^2}\right)_{\phi=0} = 2K(\cos k_x - \cos k_y). \tag{S109}$$

Using these expressions one can see that

$$\left(\frac{\partial^2 \epsilon_{\boldsymbol{k}}(\phi)}{\partial \phi^2}\right)_{\phi=0} = 2K(\cos k_x - \cos k_y)\left[\frac{A_{\boldsymbol{k}}(0) - B_{\boldsymbol{k}}(0)}{A_{\boldsymbol{k}}(0) + B_{\boldsymbol{k}}(0)}\right]^{1/2}. \tag{S110}$$

The appropriate curvature of the zero-point energy is then given by the integral

$$A_{\phi\phi} \equiv \frac{S}{2}\int_{-\pi}^{\pi}\frac{dk_x}{2\pi}\int_{-\pi}^{\pi}\frac{dk_y}{2\pi}\left(\frac{\partial^2 \epsilon_{\boldsymbol{k}}(\phi)}{\partial \phi^2}\right)_{\phi=0}. \tag{S111}$$

While still not analytically tractable, we can go further if we consider a formal expansion in $\kappa \equiv |K|/|J|$, which then renders the required integrals independent of $K$ and $J$. For example, the coefficient of the $\kappa^2$ term is given by

$$\frac{|J|S}{2}\int_{-\pi}^{\pi}\frac{dk_x}{2\pi}\int_{-\pi}^{\pi}\frac{dk_y}{2\pi}\left[\frac{\cos k_y\left(\cos k_y - \cos k_x\right)}{2 - \cos k_x - \cos k_y}\right] = \left(\frac{2}{\pi} - \frac{1}{2}\right)|J|S. \tag{S112}$$

We can do a similar integral for the next order, finding then that

$$A_{\phi\phi} = |J|S\left[\left(\frac{2}{\pi} - \frac{1}{2}\right)\kappa^2 + \left(\frac{1}{2} - \frac{27}{16\pi}\right)\kappa^3 + O(\kappa^4)\right]. \tag{S113}$$

This is in very good agreement with fitting a polynomial to the zero-point energy at small $\phi$ (see Fig. S2). For $\kappa \ll 1$, one thus finds that the pseudo-Goldstone gap is given by

$$\Delta = \frac{1}{S}\sqrt{A_{\theta\theta}A_{\phi\phi}} = \left[\frac{4}{\pi} - 1\right]^{1/2} \frac{S^{1/2}|K|^{3/2}}{|J|^{1/2}} + O(|K|^2/|J|) \approx 0.522723\, S^{1/2}\frac{|K|^{3/2}}{|J|^{1/2}}, \tag{S114}$$

as quoted in Table I of the main text.

---


[1] J.-P. Blaizot and G. Ripka, *Quantum theory of finite systems*, Vol. 3 (MIT press Cambridge, 1986).

[2] M. E. Zhitomirsky and A. L. Chernyshev, Rev. Mod. Phys. **85**, 219 (2013).

[3] V. Viswanath and G. Müller, *The Recursion Method: Application to Many Body Dynamics*, Vol. 23 (Springer Science & Business Media, 1994).

[4] G. Rickayzen, *Green's functions and condensed matter* (Courier Corporation, 2013).

[5] S. Weinberg, *The quantum theory of fields*, Vol. 2 (Cambridge university press, 1995).

[6] R. Dashen, Phys. Rev. **183**, 1245 (1969).

[7] M. Gell-Mann, R. J. Oakes, and B. Renner, Phys. Rev. **175**, 2195 (1968).

[8] E. Witten, Nuclear Physics B **156**, 269 (1979).

[9] G. Veneziano, Nuclear Physics B **159**, 213 (1979).

[10] J. R. Tessman, Phys. Rev. **96**, 1192 (1954).

[11] E. Belorizky, R. Casalegno, and J. Niez, physica status solidi (b) **102**, 365 (1980).

[12] J. Villain, R. Bidaux, J.-P. Carton, and R. Conte, Journal de Physique **41**, 1263 (1980).

[13] C. L. Henley, Phys. Rev. Lett. **62**, 2056 (1989).

[14] E. Shender, Sov. Phys. JETP **56**, 178 (1982).

[15] J. Chaloupka, G. Jackeli, and G. Khaliullin, Phys. Rev. Lett. **105**, 027204 (2010).

[16] J. G. Rau, E. K.-H. Lee, and H.-Y. Kee, Phys. Rev. Lett. **112**, 077204 (2014).

[17] J. Chaloupka, G. Jackeli, and G. Khaliullin, Phys. Rev. Lett. **110**, 097204 (2013).

[18] P. Chandra and B. Doucot, Phys. Rev. B **38**, 9335 (1988).

[19] E. Dagotto and A. Moreo, Phys. Rev. Lett. **63**, 2148 (1989).

[20] M. P. Gelfand, R. R. P. Singh, and D. A. Huse, Phys. Rev. B **40**, 10801 (1989).

[21] F. Figueirido, A. Karlhede, S. Kivelson, S. Sondhi, M. Rocek, and D. S. Rokhsar, Phys. Rev. B **41**, 4619 (1990).

[22] R. R. P. Singh and R. Narayanan, Phys. Rev. Lett. **65**, 1072 (1990).

[23] K. Sano, I. Doi, and K. Takano, Journal of the Physical Society of Japan **60**, 3807 (1991).

[24] N. Read and S. Sachdev, Phys. Rev. Lett. **66**, 1773 (1991).

[25] J. Oitmaa and Z. Weihong, Phys. Rev. B **54**, 3022 (1996).

[26] R. R. P. Singh, Z. Weihong, C. J. Hamer, and J. Oitmaa, Phys. Rev. B **60**, 7278 (1999).

[27] L. Capriotti and S. Sorella, Phys. Rev. Lett. **84**, 3173 (2000).

[28] O. P. Sushkov, J. Oitmaa, and Z. Weihong, Phys. Rev. B **63**, 104420 (2001).

[29] M. Mambrini, A. Läuchli, D. Poilblanc, and F. Mila, Phys. Rev. B **74**, 144422 (2006).

[30] R. Darradi, O. Derzhko, R. Zinke, J. Schulenburg, S. E. Krüger, and J. Richter, Phys. Rev. B **78**, 214415 (2008).

[31] H.-C. Jiang, H. Yao, and L. Balents, Phys. Rev. B **86**, 024424 (2012).

[32] W.-J. Hu, F. Becca, A. Parola, and S. Sorella, Phys. Rev. B **88**, 060402 (2013).

[33] S.-S. Gong, W. Zhu, D. N. Sheng, O. I. Motrunich, and M. P. A. Fisher, Phys. Rev. Lett. **113**, 027201 (2014).

[34] S. Morita, R. Kaneko, and M. Imada, Journal of the Physical Society of Japan **84**, 024720 (2015).

[35] R. R. P. Singh, W. Zheng, J. Oitmaa, O. P. Sushkov, and C. J. Hamer, Phys. Rev. Lett. **91**, 017201 (2003).

[36] A. V. Chubukov and T. Jolicoeur, Phys. Rev. B **46**, 11137 (1992).

[37] J. E. Hirsch and S. Tang, Phys. Rev. B **39**, 2887 (1989).

[38] R. Deutscher and H. Everts, Zeitschrift für Physik B Condensed Matter **93**, 77 (1993).

[39] P. Lecheminant, B. Bernu, C. Lhuillier, and L. Pierre, Phys. Rev. B **52**, 6647 (1995).

[40] L. O. Manuel and H. A. Ceccatto, Phys. Rev. B **60**, 9489 (1999).

[41] R. Kaneko, S. Morita, and M. Imada, Journal of the Physical Society of Japan **83**, 093707 (2014).

[42] P. H. Y. Li, R. F. Bishop, and C. E. Campbell, Phys. Rev. B **91**, 014426 (2015).

[43] Z. Zhu and S. R. White, Phys. Rev. B **92**, 041105 (2015).

[44] W.-J. Hu, S.-S. Gong, W. Zhu, and D. N. Sheng, Phys. Rev. B **92**, 140403 (2015).

[45] Y. Iqbal, W.-J. Hu, R. Thomale, D. Poilblanc, and F. Becca, Phys. Rev. B **93**, 144411 (2016).

[46] S. N. Saadatmand and I. P. McCulloch, Phys. Rev. B **94**, 121111 (2016).

[47] S. N. Saadatmand and I. P. McCulloch, Phys. Rev. B **96**, 075117 (2017).

[48] T. Jolicoeur, E. Dagotto, E. Gagliano, and S. Bacci, Phys. Rev. B **42**, 4800 (1990).

[49] T. Brueckel, B. Dorner, A. Gukasov, V. Plakhty, W. Prandl, E. Shender, and O. Smirnow, Zeitschrift für Physik B Condensed Matter **72**, 477 (1988).

[50] A. Gukasov, T. Brückel, B. Dorner, V. Plakhty, W. Prandl, E. Shender, and O. Smirnov, EPL (Europhysics Letters) **7**, 83 (1988).

[51] T. Brückel, B. Dorner, A. Gukasov, V. Plakhty, W. Prandl, E. Shender, and O. Smirnov, Physica B: Condensed Matter **156**, 308 (1989).

[52] T. Brückel, B. Dorner, A. Gukasov, and V. Plakhty, Physics Letters A **162**, 357 (1992).

[53] L. Savary, K. A. Ross, B. D. Gaulin, J. P. C. Ruff, and L. Balents, Phys. Rev. Lett. **109**, 167201 (2012).

[54] E. Lhotel, J. Robert, E. Ressouche, F. Damay, I. Mirebeau, J. Ollivier, H. Mutka, P. Dalmas de Réotier, A. Yaouanc, C. Marin, C. Decorse, and S. Petit, Phys. Rev. B **95**, 134426 (2017).

[55] K. A. Ross, Y. Qiu, J. R. D. Copley, H. A. Dabkowska, and B. D. Gaulin, Phys. Rev. Lett. **112**, 057201 (2014).
